# Supplementary material for: Scalarizing Functions in Bayesian Multiobjective Optimization
Source: arXiv:1904.05760 source file (2019-04-11)
Supplement: Supplementary file 1 [file Supplementary_material_SCF_Surrogates.pdf]

# Supplementary material - Scalarizing Functions in Expensive Multi- and Many-objective Optimization

Tinkle Chugh

Department of Computer Science, University of Exeter, UK

## 1 IGD and Hypervolume values of WFG problems

We present the best, statistically similar to the best and the worst IGD and hypervolume values of WFG problems in Tables 1 and 2 respectively. The results are similar to our observations and analyis in the main manuscript.

## 2 Hypervolume on DTLZ problems

The hypervolume values of DTLZ problems are given in Table 3.

## 3 Approximated Pareto fronts

In this section, we plot the approximated Pareto fronts on DTLZ problems of the run with the best IGD value with different number of objectives. For two and three objectives, we used scatter plots and for five and 10 objectives, we used parallel coordinates plots. As can be seen in the plots that approximated Pareto fronts in using some scalarizing functions are closer to the actual Pareto fronts than some other functions. These plots resembles with our analysis of IGD and hypervolume values provided in main manuscript.

### 3.1 Two objectives DTLZ problems

The scatter plots of the approximated Pareto fronts of two objectives DTLZ problems are shown in Figures 1-4.

| Problem | k | WS | EWC | WPO | WN | WPR | TCH | ATCH | MTCH |
|---|---|---|---|---|---|---|---|---|---|
| WFG1 | 2 | **1.31** (0.00) | 1.68 (0.30) | **1.30** (0.01) | **1.31** (0.01) | **1.31** (0.01) | **1.31** (0.00) | **1.30** (0.01) | **1.31** (0.00) |
| | 3 | **1.55** (0.01) | 1.82 (0.18) | **1.55** (0.01) | **1.55** (0.01) | **1.56** (0.01) | **1.55** (0.01) | **1.55** (0.01) | **1.55** (0.01) |
| | 5 | **2.05** (0.01) | 2.36 (0.09) | **2.04** (0.02) | **2.05** (0.01) | **2.07** (0.01) | **2.04** (0.02) | **2.05** (0.01) | **2.05** (0.01) |
| | 10 | **3.12** (0.03) | 3.58 (0.22) | **3.13** (0.04) | **3.10** (0.03) | **3.12** (0.04) | **3.11** (0.04) | **3.10** (0.04) | **3.11** (0.03) |
| WFG2 | 2 | **0.38** (0.10) | 0.46 (0.07) | **0.37** (0.07) | **0.29** (0.07) | **0.34** (0.06) | **0.37** (0.07) | **0.39** (0.06) | **0.38** (0.06) |
| | 3 | 0.71 (0.09) | 0.75 (0.07) | 0.67 (0.05) | 0.68 (0.08) | 0.74 (0.06) | 0.72 (0.08) | 0.70 (0.08) | 0.71 (0.08) |
| | 5 | **1.26** (0.20) | 1.74 (0.25) | **1.30** (0.17) | **1.25** (0.22) | **1.46** (0.09) | **1.28** (0.23) | **1.26** (0.13) | **1.22** (0.19) |
| | 10 | **3.67** (0.34) | 4.23 (0.61) | **3.86** (0.44) | **3.34** (0.64) | **3.81** (0.41) | **4.04** (0.50) | **3.85** (0.46) | **3.96** (0.32) |
| WFG3 | 2 | 0.31 (0.05) | 0.49 (0.06) | 0.26 (0.03) | 0.25 (0.02) | 0.37 (0.05) | 0.32 (0.02) | 0.31 (0.02) | 0.32 (0.03) |
| | 3 | 0.49 (0.04) | 0.54 (0.06) | 0.38 (0.04) | 0.48 (0.02) | 0.55 (0.03) | 0.52 (0.03) | 0.52 (0.03) | 0.52 (0.04) |
| | 5 | 0.70 (0.04) | 0.76 (0.05) | 0.64 (0.05) | 0.68 (0.05) | 0.71 (0.05) | 0.71 (0.04) | 0.70 (0.04) | 0.71 (0.05) |
| | 10 | 1.04 (0.08) | 1.15 (0.08) | **0.87** (0.09) | 1.03 (0.11) | 1.06 (0.12) | 1.07 (0.10) | 1.06 (0.11) | 1.06 (0.09) |
| WFG4 | 2 | **0.21** (0.02) | 0.40 (0.09) | **0.26** (0.05) | **0.21** (0.03) | **0.21** (0.03) | **0.26** (0.04) | **0.25** (0.06) | **0.24** (0.04) |
| | 3 | **0.56** (0.05) | 0.81 (0.16) | **0.62** (0.05) | **0.48** (0.04) | **0.63** (0.06) | **0.58** (0.08) | **0.62** (0.06) | **0.61** (0.04) |
| | 5 | **1.64** (0.22) | 2.45 (0.27) | **1.69** (0.13) | **1.51** (0.14) | **1.69** (0.07) | **1.78** (0.13) | **1.81** (0.10) | **1.82** (0.24) |
| | 10 | 7.32 (0.50) | 10.43 (0.96) | 7.60 (0.29) | **6.50** (0.29) | **7.08** (0.45) | 7.82 (0.47) | 7.68 (0.40) | 7.97 (0.38) |
| WFG5 | 2 | **0.28** (0.04) | 0.64 (0.05) | 0.38 (0.04) | **0.29** (0.05) | 0.37 (0.04) | 0.40 (0.05) | 0.39 (0.05) | 0.40 (0.06) |
| | 3 | **0.72** (0.09) | 0.93 (0.06) | 0.78 (0.11) | **0.71** (0.09) | 0.80 (0.09) | 0.76 (0.07) | 0.76 (0.05) | 0.75 (0.06) |
| | 5 | 2.33 (0.12) | 2.39 (0.14) | 2.25 (0.11) | 2.36 (0.13) | 2.48 (0.18) | 2.29 (0.19) | 2.32 (0.20) | 2.34 (0.16) |
| | 10 | 9.27 (0.29) | 9.13 (0.39) | 9.07 (0.33) | 9.26 (0.27) | 9.22 (0.23) | 9.15 (0.32) | 9.10 (0.36) | 9.21 (0.28) |
| WFG6 | 2 | 0.40 (0.06) | 0.57 (0.08) | 0.39 (0.05) | 0.35 (0.06) | 0.41 (0.04) | 0.42 (0.03) | 0.42 (0.04) | 0.44 (0.04) |
| | 3 | 0.69 (0.02) | 0.88 (0.08) | 0.69 (0.03) | 0.71 (0.03) | 0.73 (0.04) | 0.69 (0.02) | 0.68 (0.02) | 0.69 (0.02) |
| | 5 | 1.65 (0.09) | 2.07 (0.09) | 1.63 (0.04) | 1.77 (0.08) | 1.67 (0.07) | **1.58** (0.04) | **1.57** (0.05) | **1.57** (0.04) |
| | 10 | 8.14 (0.50) | 8.71 (0.31) | 8.52 (0.24) | 8.62 (0.31) | **7.62** (0.39) | **7.43** (0.48) | **7.58** (0.43) | **7.61** (0.40) |
| WFG7 | 2 | 0.42 (0.06) | 0.50 (0.06) | 0.27 (0.03) | 0.37 (0.06) | 0.43 (0.03) | 0.38 (0.01) | 0.38 (0.02) | 0.37 (0.02) |
| | 3 | 0.79 (0.03) | 0.90 (0.09) | 0.73 (0.04) | 0.77 (0.04) | 0.78 (0.02) | 0.79 (0.04) | 0.78 (0.05) | 0.77 (0.03) |
| | 5 | 2.18 (0.16) | 2.58 (0.16) | 2.20 (0.11) | 2.31 (0.24) | 2.25 (0.10) | 2.20 (0.12) | 2.15 (0.07) | 2.21 (0.12) |
| | 10 | 10.09 (0.35) | 10.17 (0.30) | **9.75** (0.28) | 10.16 (0.42) | 10.10 (0.43) | **9.57** (0.39) | **9.59** (0.34) | **9.83** (0.49) |
| WFG8 | 2 | **0.68** (0.05) | 0.84 (0.10) | **0.71** (0.05) | **0.72** (0.06) | **0.65** (0.04) | **0.70** (0.03) | **0.67** (0.03) | **0.69** (0.03) |
| | 3 | **0.99** (0.02) | 1.13 (0.10) | **0.92** (0.03) | **0.99** (0.03) | **0.97** (0.02) | **0.97** (0.02) | **0.97** (0.02) | **0.96** (0.02) |
| | 5 | 2.35 (0.13) | 2.78 (0.19) | 2.24 (0.12) | 2.51 (0.16) | 2.23 (0.09) | 2.27 (0.10) | 2.25 (0.11) | 2.28 (0.15) |
| | 10 | 9.80 (0.37) | 10.07 (0.25) | 9.49 (0.52) | 9.95 (0.32) | 9.75 (0.49) | 9.58 (0.39) | 9.51 (0.43) | 9.55 (0.52) |
| WFG9 | 2 | **0.26** (0.07) | 0.49 (0.08) | 0.35 (0.07) | 0.29 (0.11) | 0.33 (0.12) | 0.34 (0.10) | 0.35 (0.07) | 0.36 (0.07) |
| | 3 | **0.62** (0.10) | 0.91 (0.06) | 0.70 (0.07) | 0.70 (0.08) | 0.79 (0.06) | 0.68 (0.11) | 0.67 (0.07) | 0.66 (0.07) |
| | 5 | 2.35 (0.12) | 2.35 (0.15) | 2.33 (0.16) | 2.48 (0.23) | 2.42 (0.14) | 2.24 (0.17) | 2.33 (0.17) | 2.29 (0.12) |
| | 10 | **9.26** (0.25) | **9.13** (0.34) | **9.20** (0.22) | **9.22** (0.19) | **9.22** (0.30) | **9.19** (0.26) | **9.22** (0.21) | **9.23** (0.25) |

| Problem | k | PBI | IPBI | HypI | DomRank | MSD | QPBI | APD |
|---|---|---|---|---|---|---|---|---|
| WFG1 | 2 | **1.29** (0.03) | **1.31** (0.01) | **1.39** (0.32) | **1.29** (0.02) | **1.33** (0.04) | **1.42** (0.08) | **1.34** (0.03) |
| | 3 | **1.57** (0.03) | **1.67** (0.10) | 2.10 (0.40) | **1.55** (0.02) | **1.55** (0.03) | **1.73** (0.09) | **1.59** (0.02) |
| | 5 | **2.19** (0.14) | 2.28 (0.10) | 2.72 (0.30) | **2.20** (0.07) | **2.14** (0.20) | 2.39 (0.19) | **2.19** (0.06) |
| | 10 | 3.42 (0.09) | 3.38 (0.05) | 4.01 (0.10) | 3.46 (0.27) | 3.56 (0.22) | 3.90 (0.22) | 3.72 (0.18) |
| WFG2 | 2 | **0.29** (0.08) | 0.43 (0.06) | **0.30** (0.08) | **0.36** (0.06) | **0.30** (0.04) | **0.38** (0.07) | **0.40** (0.06) |
| | 3 | **0.62** (0.08) | 0.78 (0.07) | 0.82 (0.06) | 0.67 (0.08) | **0.54** (0.07) | 0.75 (0.08) | 0.67 (0.08) |
| | 5 | **1.34** (0.45) | 1.71 (0.21) | 1.80 (0.24) | **1.40** (0.27) | **1.39** (0.42) | **1.65** (0.27) | **1.41** (0.45) |
| | 10 | **3.36** (0.86) | 4.29 (0.47) | 4.34 (0.44) | **4.19** (0.27) | 4.25 (0.57) | **4.18** (0.64) | 4.32 (0.45) |
| WFG3 | 2 | 0.35 (0.03) | 0.44 (0.03) | **0.15** (0.05) | 0.37 (0.04) | 0.23 (0.03) | 0.31 (0.03) | 0.24 (0.03) |
| | 3 | 0.40 (0.04) | 0.56 (0.03) | **0.27** (0.09) | 0.46 (0.05) | 0.39 (0.05) | **0.34** (0.05) | 0.37 (0.06) |
| | 5 | **0.35** (0.06) | 0.66 (0.06) | 0.52 (0.18) | 0.63 (0.04) | **0.42** (0.06) | **0.38** (0.06) | **0.34** (0.06) |
| | 10 | **0.79** (0.09) | 1.05 (0.08) | 1.10 (0.11) | 1.05 (0.13) | 0.97 (0.11) | **0.85** (0.05) | **0.86** (0.11) |
| WFG4 | 2 | **0.19** (0.03) | 0.32 (0.09) | **0.26** (0.13) | 0.31 (0.02) | **0.28** (0.07) | 0.34 (0.12) | 0.35 (0.10) |
| | 3 | **0.46** (0.06) | 0.67 (0.10) | 0.68 (0.25) | 0.68 (0.08) | 0.70 (0.13) | 0.87 (0.20) | **0.45** (0.06) |
| | 5 | **1.52** (0.16) | 2.39 (0.19) | 3.00 (0.30) | 2.50 (0.37) | 2.72 (0.42) | 2.82 (0.25) | **1.59** (0.17) |
| | 10 | 9.84 (0.64) | 10.37 (0.27) | 11.89 (0.34) | 11.67 (0.54) | 11.84 (0.34) | 8.00 (0.47) | 9.71 (0.46) |
| WFG5 | 2 | 0.32 (0.03) | 0.48 (0.05) | **0.20** (0.06) | **0.26** (0.06) | 0.34 (0.05) | 0.47 (0.07) | 0.44 (0.08) |
| | 3 | **0.59** (0.03) | 0.81 (0.06) | **0.64** (0.15) | **0.72** (0.12) | **0.61** (0.07) | 0.73 (0.07) | **0.62** (0.08) |
| | 5 | **1.98** (0.23) | 2.30 (0.14) | 2.53 (0.15) | 2.07 (0.10) | **2.03** (0.15) | 2.25 (0.15) | **1.79** (0.10) |
| | 10 | 9.36 (0.26) | 9.12 (0.27) | 9.43 (0.27) | 9.39 (0.28) | **8.37** (0.46) | 9.32 (0.25) | 9.14 (0.26) |
| WFG6 | 2 | **0.29** (0.05) | 0.42 (0.04) | **0.25** (0.06) | 0.54 (0.04) | **0.31** (0.06) | 0.38 (0.07) | 0.42 (0.07) |
| | 3 | **0.57** (0.05) | 0.74 (0.05) | 0.68 (0.23) | 0.89 (0.08) | **0.63** (0.07) | **0.65** (0.11) | **0.53** (0.05) |
| | 5 | **1.41** (0.06) | 2.15 (0.10) | 2.26 (0.18) | 2.24 (0.15) | 2.16 (0.11) | 1.77 (0.19) | **1.58** (0.09) |
| | 10 | 8.74 (0.29) | 8.88 (0.19) | 8.92 (0.17) | 8.93 (0.18) | 8.79 (0.21) | 8.83 (0.22) | 8.82 (0.21) |
| WFG7 | 2 | 0.30 (0.03) | 0.43 (0.05) | **0.15** (0.05) | 0.34 (0.03) | 0.24 (0.03) | 0.32 (0.02) | 0.30 (0.04) |
| | 3 | 0.63 (0.04) | 0.77 (0.05) | **0.48** (0.08) | 0.62 (0.02) | 0.76 (0.11) | 0.63 (0.06) | 0.59 (0.04) |
| | 5 | **1.85** (0.18) | 2.36 (0.16) | 2.13 (0.21) | 2.16 (0.11) | 2.58 (0.18) | 2.40 (0.26) | **1.74** (0.12) |
| | 10 | 10.17 (0.26) | **9.34** (0.43) | 10.17 (0.42) | 10.14 (0.35) | 10.12 (0.26) | 10.16 (0.26) | **9.91** (0.30) |
| WFG8 | 2 | **0.67** (0.03) | **0.65** (0.03) | **0.66** (0.08) | **0.66** (0.04) | **0.69** (0.06) | **0.69** (0.03) | **0.69** (0.03) |
| | 3 | **0.91** (0.03) | **0.98** (0.02) | 1.14 (0.21) | **0.93** (0.11) | 1.10 (0.13) | **0.92** (0.03) | **0.89** (0.03) |
| | 5 | **2.07** (0.15) | **2.18** (0.08) | 2.92 (0.15) | 2.66 (0.30) | 2.88 (0.15) | 2.64 (0.20) | **1.96** (0.05) |
| | 10 | 10.07 (0.23) | **8.32** (0.69) | 10.12 (0.24) | 10.01 (0.32) | 10.06 (0.22) | 10.09 (0.26) | 9.76 (0.36) |
| WFG9 | 2 | **0.23** (0.07) | 0.49 (0.06) | **0.12** (0.06) | 0.48 (0.07) | 0.38 (0.12) | 0.44 (0.11) | 0.41 (0.08) |
| | 3 | **0.44** (0.10) | 0.92 (0.07) | 0.76 (0.24) | 0.71 (0.11) | **0.60** (0.14) | 0.84 (0.10) | **0.60** (0.11) |
| | 5 | **1.81** (0.14) | 2.45 (0.15) | 2.40 (0.28) | 2.28 (0.11) | **2.04** (0.16) | 2.24 (0.23) | **1.86** (0.19) |
| | 10 | **9.18** (0.24) | **9.25** (0.24) | 9.31 (0.22) | **9.21** (0.24) | **9.26** (0.24) | **9.19** (0.28) | **9.17** (0.20) |

Table 1: , Mean IGD values and standard deviation (in parentheses) for WFG problems. The values statistically similar to the best one are in bold, the best value is encircled the worst value is underlined

| Problem | k | WS | EWC | WPO | WN | WPR | TCH | ATCH | MTCH |
|---|---|---|---|---|---|---|---|---|---|
| WFG1 | 2 | **0.22** (0.00) | 0.09 (0.06) | **0.22** (0.00) | **0.22** (0.00) | **0.22** (0.00) | **0.22** (0.00) | **0.22** (0.00) | **0.22** (0.00) |
| | 3 | **0.34** (0.00) | 0.20 (0.06) | **0.34** (0.00) | **0.34** (0.00) | **0.33** (0.01) | **0.34** (0.00) | **0.34** (0.00) | **0.34** (0.00) |
| | 5 | **0.31** (0.00) | 0.23 (0.03) | **0.31** (0.00) | **0.31** (0.00) | **0.31** (0.00) | **0.31** (0.00) | **0.31** (0.00) | **0.31** (0.00) |
| | 10 | **0.24** (0.00) | 0.16 (0.03) | **0.23** (0.00) | **0.24** (0.00) | **0.23** (0.00) | **0.24** (0.00) | **0.24** (0.00) | **0.23** (0.00) |
| WFG2 | 2 | **0.49** (0.05) | 0.43 (0.03) | **0.49** (0.03) | **0.52** (0.05) | **0.50** (0.04) | **0.49** (0.03) | **0.48** (0.03) | **0.49** (0.03) |
| | 3 | **0.66** (0.05) | 0.56 (0.05) | **0.70** (0.04) | **0.70** (0.04) | 0.63 (0.02) | 0.64 (0.04) | 0.64 (0.03) | 0.64 (0.03) |
| | 5 | **0.77** (0.06) | 0.60 (0.06) | **0.72** (0.05) | **0.79** (0.05) | 0.68 (0.04) | **0.73** (0.05) | **0.72** (0.03) | **0.72** (0.04) |
| | 10 | **0.76** (0.07) | 0.58 (0.06) | **0.70** (0.06) | **0.80** (0.05) | 0.67 (0.06) | 0.68 (0.09) | 0.68 (0.08) | **0.70** (0.06) |
| WFG3 | 2 | 0.49 (0.02) | 0.41 (0.02) | 0.51 (0.02) | 0.52 (0.01) | 0.46 (0.03) | 0.49 (0.01) | 0.49 (0.01) | 0.49 (0.01) |
| | 3 | 0.29 (0.02) | 0.26 (0.03) | 0.31 (0.01) | 0.29 (0.01) | 0.26 (0.01) | 0.27 (0.01) | 0.27 (0.01) | 0.27 (0.01) |
| | 5 | 0.13 (0.02) | 0.11 (0.02) | 0.14 (0.02) | 0.13 (0.02) | 0.13 (0.02) | 0.12 (0.02) | 0.12 (0.02) | 0.11 (0.02) |
| | 10 | 0.03 (0.01) | 0.02 (0.01) | **0.04** (0.01) | **0.04** (0.01) | 0.03 (0.01) | 0.03 (0.01) | 0.03 (0.01) | 0.03 (0.01) |
| WFG4 | 2 | **0.35** (0.01) | 0.27 (0.02) | **0.33** (0.01) | **0.35** (0.02) | **0.35** (0.01) | **0.33** (0.01) | **0.33** (0.01) | **0.32** (0.02) |
| | 3 | **0.46** (0.01) | 0.33 (0.03) | 0.40 (0.03) | **0.48** (0.01) | 0.40 (0.01) | 0.41 (0.02) | 0.42 (0.02) | 0.42 (0.02) |
| | 5 | **0.55** (0.04) | 0.33 (0.02) | 0.44 (0.03) | **0.59** (0.03) | 0.42 (0.02) | 0.44 (0.03) | 0.45 (0.04) | 0.45 (0.03) |
| | 10 | 0.40 (0.04) | 0.28 (0.02) | 0.37 (0.04) | **0.52** (0.02) | 0.33 (0.04) | 0.35 (0.04) | 0.36 (0.04) | 0.33 (0.03) |
| WFG5 | 2 | 0.29 (0.02) | 0.20 (0.01) | 0.27 (0.01) | 0.29 (0.02) | 0.28 (0.01) | 0.26 (0.01) | 0.26 (0.01) | 0.27 (0.01) |
| | 3 | **0.34** (0.03) | 0.26 (0.01) | 0.33 (0.03) | **0.36** (0.03) | **0.34** (0.02) | 0.33 (0.02) | 0.32 (0.02) | 0.33 (0.02) |
| | 5 | 0.30 (0.02) | 0.26 (0.01) | 0.31 (0.02) | 0.31 (0.02) | 0.28 (0.02) | 0.31 (0.02) | 0.31 (0.02) | 0.31 (0.01) |
| | 10 | **0.28** (0.02) | 0.24 (0.01) | 0.25 (0.02) | **0.28** (0.01) | 0.26 (0.02) | **0.28** (0.01) | **0.28** (0.02) | **0.27** (0.02) |
| WFG6 | 2 | 0.24 (0.03) | 0.21 (0.02) | 0.26 (0.02) | 0.27 (0.03) | 0.24 (0.03) | 0.23 (0.02) | 0.23 (0.02) | 0.23 (0.02) |
| | 3 | 0.30 (0.01) | 0.27 (0.02) | 0.33 (0.02) | 0.32 (0.03) | 0.30 (0.02) | 0.30 (0.01) | 0.31 (0.01) | 0.31 (0.01) |
| | 5 | 0.39 (0.02) | 0.28 (0.01) | 0.39 (0.01) | 0.36 (0.02) | 0.39 (0.02) | 0.40 (0.01) | 0.40 (0.01) | 0.40 (0.01) |
| | 10 | 0.29 (0.02) | 0.25 (0.01) | 0.28 (0.02) | 0.27 (0.02) | **0.32** (0.02) | **0.32** (0.03) | **0.32** (0.02) | **0.32** (0.02) |
| WFG7 | 2 | 0.28 (0.03) | 0.24 (0.01) | 0.31 (0.01) | 0.32 (0.02) | 0.25 (0.02) | 0.26 (0.01) | 0.26 (0.01) | 0.26 (0.01) |
| | 3 | 0.32 (0.02) | 0.30 (0.02) | **0.42** (0.02) | 0.36 (0.04) | 0.32 (0.03) | 0.32 (0.02) | 0.33 (0.01) | 0.33 (0.01) |
| | 5 | 0.30 (0.03) | 0.29 (0.01) | 0.29 (0.01) | 0.31 (0.01) | 0.29 (0.02) | 0.28 (0.01) | 0.28 (0.01) | 0.28 (0.02) |
| | 10 | 0.27 (0.01) | 0.28 (0.01) | 0.28 (0.01) | 0.27 (0.02) | 0.27 (0.01) | 0.27 (0.01) | 0.26 (0.01) | 0.27 (0.01) |
| WFG8 | 2 | 0.17 (0.01) | 0.16 (0.01) | 0.17 (0.01) | 0.16 (0.01) | 0.17 (0.02) | 0.16 (0.01) | 0.16 (0.01) | 0.16 (0.01) |
| | 3 | 0.22 (0.02) | 0.21 (0.02) | **0.25** (0.01) | 0.23 (0.03) | **0.24** (0.02) | **0.23** (0.01) | **0.24** (0.01) | **0.25** (0.01) |
| | 5 | 0.24 (0.01) | 0.23 (0.02) | 0.27 (0.01) | 0.24 (0.02) | 0.24 (0.01) | 0.24 (0.01) | 0.23 (0.01) | 0.24 (0.01) |
| | 10 | 0.23 (0.01) | 0.24 (0.01) | 0.24 (0.01) | 0.23 (0.01) | 0.24 (0.01) | **0.25** (0.01) | 0.24 (0.01) | 0.24 (0.01) |
| WFG9 | 2 | 0.33 (0.02) | 0.24 (0.03) | 0.30 (0.02) | 0.30 (0.04) | 0.29 (0.04) | 0.30 (0.03) | 0.29 (0.02) | 0.29 (0.02) |
| | 3 | **0.38** (0.05) | 0.27 (0.02) | 0.36 (0.02) | 0.35 (0.03) | 0.33 (0.03) | 0.36 (0.04) | 0.36 (0.03) | 0.37 (0.03) |
| | 5 | 0.30 (0.03) | 0.27 (0.02) | 0.29 (0.02) | 0.28 (0.04) | 0.28 (0.02) | 0.31 (0.03) | 0.30 (0.02) | 0.30 (0.02) |
| | 10 | 0.28 (0.02) | 0.27 (0.01) | 0.27 (0.01) | 0.29 (0.02) | 0.26 (0.01) | 0.28 (0.01) | 0.28 (0.01) | 0.27 (0.01) |

| Problem | k | PBI | IPBI | HypI | DomRank | MSD | QPBI | APD |
|---|---|---|---|---|---|---|---|---|
| WFG1 | 2 | **0.23** (0.01) | **0.22** (0.00) | **0.19** (0.07) | **0.21** (0.01) | **0.20** (0.02) | 0.15 (0.03) | **0.19** (0.02) |
| | 3 | **0.31** (0.02) | 0.28 (0.04) | 0.15 (0.13) | **0.32** (0.01) | **0.34** (0.01) | 0.25 (0.02) | **0.31** (0.02) |
| | 5 | **0.27** (0.04) | 0.26 (0.03) | 0.14 (0.08) | **0.28** (0.01) | **0.30** (0.03) | 0.21 (0.07) | **0.28** (0.02) |
| | 10 | 0.18 (0.03) | **0.21** (0.02) | 0.11 (0.06) | **0.22** (0.02) | 0.18 (0.03) | 0.10 (0.06) | 0.15 (0.04) |
| WFG2 | 2 | **0.52** (0.04) | 0.46 (0.03) | **0.50** (0.04) | **0.48** (0.03) | **0.50** (0.03) | **0.47** (0.03) | **0.47** (0.03) |
| | 3 | 0.63 (0.05) | 0.60 (0.04) | 0.53 (0.03) | 0.64 (0.05) | **0.73** (0.05) | 0.60 (0.06) | 0.64 (0.06) |
| | 5 | **0.73** (0.11) | **0.70** (0.06) | 0.59 (0.04) | **0.71** (0.05) | **0.73** (0.10) | 0.67 (0.06) | **0.73** (0.10) |
| | 10 | **0.77** (0.09) | 0.65 (0.06) | 0.57 (0.05) | 0.60 (0.03) | 0.64 (0.06) | 0.66 (0.07) | 0.63 (0.06) |
| WFG3 | 2 | 0.47 (0.01) | 0.42 (0.02) | **0.56** (0.02) | 0.45 (0.02) | 0.52 (0.01) | 0.48 (0.01) | 0.53 (0.02) |
| | 3 | 0.32 (0.02) | 0.26 (0.02) | **0.36** (0.03) | 0.28 (0.01) | 0.31 (0.02) | 0.33 (0.02) | 0.33 (0.03) |
| | 5 | **0.21** (0.02) | 0.14 (0.02) | 0.16 (0.04) | 0.12 (0.02) | **0.19** (0.03) | **0.19** (0.02) | **0.21** (0.02) |
| | 10 | **0.06** (0.01) | 0.03 (0.01) | 0.02 (0.01) | 0.02 (0.01) | 0.02 (0.01) | **0.05** (0.01) | **0.04** (0.02) |
| WFG4 | 2 | **0.34** (0.02) | 0.29 (0.03) | **0.34** (0.03) | 0.28 (0.01) | 0.32 (0.03) | 0.29 (0.02) | 0.29 (0.02) |
| | 3 | **0.46** (0.03) | 0.36 (0.03) | 0.40 (0.07) | 0.35 (0.03) | 0.38 (0.04) | 0.33 (0.05) | **0.44** (0.04) |
| | 5 | **0.59** (0.03) | 0.37 (0.04) | 0.31 (0.04) | 0.32 (0.02) | 0.35 (0.03) | 0.32 (0.02) | 0.48 (0.06) |
| | 10 | 0.39 (0.02) | 0.35 (0.02) | 0.25 (0.01) | 0.25 (0.01) | 0.26 (0.01) | 0.42 (0.02) | 0.36 (0.01) |
| WFG5 | 2 | 0.28 (0.01) | 0.22 (0.02) | **0.35** (0.02) | **0.33** (0.02) | 0.30 (0.01) | 0.23 (0.02) | 0.24 (0.03) |
| | 3 | **0.35** (0.02) | 0.28 (0.02) | **0.36** (0.06) | 0.34 (0.04) | **0.38** (0.03) | 0.30 (0.03) | **0.35** (0.03) |
| | 5 | **0.38** (0.02) | 0.27 (0.01) | 0.25 (0.02) | 0.29 (0.02) | 0.30 (0.02) | 0.28 (0.01) | 0.34 (0.02) |
| | 10 | **0.30** (0.02) | 0.24 (0.01) | 0.23 (0.01) | 0.23 (0.01) | 0.24 (0.01) | **0.27** (0.02) | 0.27 (0.01) |
| WFG6 | 2 | **0.31** (0.01) | 0.24 (0.02) | **0.33** (0.03) | 0.22 (0.02) | **0.30** (0.03) | 0.27 (0.03) | 0.26 (0.02) |
| | 3 | **0.41** (0.02) | 0.31 (0.02) | 0.36 (0.08) | 0.26 (0.02) | 0.36 (0.02) | 0.35 (0.05) | **0.42** (0.03) |
| | 5 | **0.50** (0.04) | 0.31 (0.01) | 0.27 (0.04) | 0.28 (0.02) | 0.29 (0.02) | 0.37 (0.06) | 0.44 (0.03) |
| | 10 | **0.31** (0.03) | 0.26 (0.01) | 0.23 (0.01) | 0.23 (0.01) | 0.25 (0.01) | 0.29 (0.02) | 0.26 (0.01) |
| WFG7 | 2 | 0.29 (0.01) | 0.24 (0.01) | **0.37** (0.02) | 0.29 (0.02) | **0.35** (0.02) | 0.28 (0.01) | 0.30 (0.02) |
| | 3 | 0.39 (0.02) | 0.31 (0.02) | **0.45** (0.03) | 0.37 (0.01) | 0.35 (0.03) | 0.38 (0.03) | 0.39 (0.02) |
| | 5 | **0.44** (0.03) | 0.32 (0.02) | 0.37 (0.04) | 0.34 (0.01) | 0.32 (0.01) | 0.33 (0.05) | **0.44** (0.03) |
| | 10 | 0.29 (0.02) | **0.33** (0.01) | 0.29 (0.02) | 0.30 (0.01) | 0.30 (0.02) | 0.29 (0.02) | 0.30 (0.02) |
| WFG8 | 2 | 0.16 (0.01) | 0.17 (0.01) | **0.21** (0.01) | 0.18 (0.01) | 0.17 (0.01) | 0.16 (0.01) | 0.17 (0.01) |
| | 3 | **0.26** (0.01) | **0.24** (0.02) | 0.23 (0.04) | **0.23** (0.01) | **0.24** (0.02) | **0.25** (0.02) | **0.26** (0.02) |
| | 5 | **0.31** (0.03) | 0.26 (0.02) | 0.22 (0.03) | 0.24 (0.02) | 0.23 (0.01) | 0.25 (0.02) | 0.27 (0.02) |
| | 10 | 0.24 (0.01) | **0.26** (0.02) | 0.23 (0.01) | 0.24 (0.01) | 0.23 (0.01) | 0.24 (0.01) | **0.25** (0.01) |
| WFG9 | 2 | **0.34** (0.02) | 0.25 (0.02) | **0.38** (0.02) | 0.25 (0.02) | 0.29 (0.05) | 0.26 (0.04) | 0.27 (0.03) |
| | 3 | **0.43** (0.04) | 0.26 (0.02) | 0.34 (0.09) | 0.35 (0.04) | **0.39** (0.04) | 0.29 (0.03) | **0.38** (0.04) |
| | 5 | **0.44** (0.01) | 0.26 (0.01) | 0.28 (0.06) | 0.30 (0.02) | 0.34 (0.03) | 0.30 (0.03) | 0.37 (0.03) |
| | 10 | **0.32** (0.02) | 0.27 (0.02) | 0.26 (0.01) | 0.27 (0.01) | 0.27 (0.01) | **0.30** (0.02) | 0.28 (0.01) |

Table 2: Mean hypervolume values and standard deviation (in parentheses) for WFG problems. The values statistically similar to the best one are in bold, the best value is encircled the worst value is underlined

| Problem | k | WS | EWC | WPO | WN | WPR | TCH | ATCH | MTCH |
|---|---|---|---|---|---|---|---|---|---|
| DTLZ1 | 2 | 0.00 (0.00) | 0.00 (0.00) | 0.00 (0.00) | 0.00 (0.00) | 0.00 (0.00) | 0.00 (0.00) | 0.00 (0.00) | 0.00 (0.00) |
| | 3 | 0.00 (0.00) | 0.00 (0.00) | 0.00 (0.00) | 0.00 (0.00) | 0.00 (0.00) | 0.00 (0.00) | 0.00 (0.00) | 0.00 (0.00) |
| | 5 | 0.00 (0.00) | 0.00 (0.00) | 0.00 (0.00) | 0.00 (0.00) | 0.00 (0.00) | 0.00 (0.00) | 0.00 (0.00) | 0.00 (0.00) |
| | 10 | 0.00 (0.00) | 0.00 (0.00) | 0.00 (0.00) | 0.00 (0.00) | 0.00 (0.00) | 0.00 (0.00) | 0.00 (0.00) | 0.00 (0.00) |
| DTLZ2 | 2 | 0.58 (0.01) | 0.53 (0.03) | **0.64** (0.00) | 0.57 (0.01) | 0.57 (0.01) | **0.63** (0.00) | **0.63** (0.00) | **0.63** (0.00) |
| | 3 | 0.74 (0.01) | 0.67 (0.03) | **0.78** (0.00) | 0.73 (0.01) | 0.74 (0.01) | **0.78** (0.00) | **0.78** (0.00) | **0.78** (0.00) |
| | 5 | 0.88 (0.01) | 0.74 (0.04) | 0.89 (0.01) | 0.88 (0.01) | 0.89 (0.01) | 0.87 (0.01) | 0.88 (0.01) | 0.88 (0.01) |
| | 10 | **0.84** (0.03) | 0.73 (0.03) | **0.87** (0.02) | **0.85** (0.04) | 0.82 (0.03) | **0.86** (0.03) | **0.85** (0.03) | **0.85** (0.02) |
| DTLZ3 | 2 | 0.00 (0.00) | 0.00 (0.00) | 0.00 (0.00) | 0.00 (0.00) | 0.00 (0.00) | 0.00 (0.00) | 0.00 (0.00) | 0.00 (0.00) |
| | 3 | 0.00 (0.00) | 0.00 (0.00) | 0.00 (0.00) | 0.00 (0.00) | 0.00 (0.00) | 0.00 (0.00) | 0.00 (0.00) | 0.00 (0.00) |
| | 5 | 0.00 (0.00) | 0.00 (0.00) | 0.00 (0.00) | 0.00 (0.00) | 0.00 (0.00) | 0.00 (0.00) | 0.00 (0.00) | 0.00 (0.00) |
| | 10 | 0.00 (0.00) | 0.00 (0.00) | 0.00 (0.00) | 0.00 (0.00) | 0.00 (0.00) | 0.00 (0.00) | 0.00 (0.00) | 0.00 (0.00) |
| DTLZ4 | 2 | **0.54** (0.03) | 0.40 (0.08) | **0.55** (0.01) | 0.45 (0.09) | 0.38 (0.07) | **0.56** (0.01) | **0.56** (0.00) | **0.56** (0.00) |
| | 3 | 0.61 (0.07) | 0.50 (0.08) | **0.70** (0.00) | 0.48 (0.06) | 0.51 (0.08) | **0.65** (0.06) | **0.65** (0.04) | **0.67** (0.05) |
| | 5 | 0.71 (0.06) | 0.63 (0.09) | **0.85** (0.01) | 0.71 (0.06) | 0.59 (0.09) | **0.73** (0.06) | 0.69 (0.10) | 0.70 (0.10) |
| | 10 | **0.89** (0.04) | 0.82 (0.05) | **0.91** (0.03) | **0.88** (0.04) | 0.78 (0.05) | **0.90** (0.05) | **0.90** (0.03) | **0.90** (0.04) |
| DTLZ5 | 2 | 0.58 (0.01) | 0.53 (0.02) | **0.63** (0.00) | 0.57 (0.01) | 0.57 (0.01) | **0.63** (0.00) | **0.63** (0.00) | **0.63** (0.00) |
| | 3 | 0.47 (0.00) | 0.43 (0.03) | **0.52** (0.01) | 0.47 (0.00) | 0.46 (0.01) | **0.51** (0.00) | **0.51** (0.00) | **0.51** (0.01) |
| | 5 | 0.40 (0.01) | 0.34 (0.03) | **0.43** (0.00) | 0.40 (0.01) | 0.40 (0.01) | 0.42 (0.01) | 0.42 (0.01) | 0.42 (0.00) |
| | 10 | 0.36 (0.01) | 0.31 (0.03) | **0.39** (0.00) | 0.37 (0.00) | 0.37 (0.01) | 0.37 (0.00) | **0.37** (0.00) | **0.37** (0.01) |
| DTLZ6 | 2 | **0.51** (0.06) | 0.00 (0.00) | **0.48** (0.08) | **0.53** (0.04) | 0.24 (0.19) | **0.53** (0.03) | **0.53** (0.07) | **0.52** (0.07) |
| | 3 | **0.32** (0.10) | 0.00 (0.00) | 0.15 (0.10) | 0.25 (0.13) | 0.09 (0.10) | **0.34** (0.10) | **0.30** (0.09) | **0.35** (0.09) |
| | 5 | 0.05 (0.06) | 0.00 (0.00) | 0.01 (0.04) | 0.08 (0.09) | 0.01 (0.01) | 0.05 (0.08) | 0.05 (0.08) | 0.01 (0.04) |
| | 10 | 0.00 (0.00) | 0.00 (0.00) | 0.00 (0.00) | 0.00 (0.00) | 0.00 (0.00) | 0.00 (0.00) | 0.00 (0.01) | 0.00 (0.00) |
| DTLZ7 | 2 | 0.23 (0.01) | 0.00 (0.00) | 0.20 (0.03) | 0.26 (0.02) | 0.19 (0.03) | 0.23 (0.01) | 0.23 (0.02) | 0.23 (0.01) |
| | 3 | 0.21 (0.03) | 0.00 (0.00) | 0.18 (0.02) | 0.17 (0.01) | 0.17 (0.02) | 0.22 (0.01) | 0.21 (0.02) | 0.22 (0.01) |
| | 5 | **0.15** (0.00) | 0.00 (0.00) | 0.04 (0.04) | **0.15** (0.00) | 0.12 (0.02) | 0.15 (0.01) | **0.15** (0.01) | 0.15 (0.01) |
| | 10 | **0.05** (0.01) | 0.00 (0.00) | 0.00 (0.01) | **0.08** (0.01) | 0.03 (0.01) | 0.03 (0.01) | 0.05 (0.01) | 0.04 (0.01) |

| Problem | k | PBI | IPBI | HypI | DomRank | MSD | QPBI | APD |
|---|---|---|---|---|---|---|---|---|
| DTLZ1 | 2 | 0.00 (0.00) | 0.00 (0.00) | 0.00 (0.00) | 0.00 (0.00) | 0.00 (0.00) | 0.00 (0.00) | 0.00 (0.00) |
| | 3 | 0.00 (0.00) | 0.00 (0.00) | 0.00 (0.00) | 0.00 (0.00) | 0.00 (0.00) | 0.00 (0.00) | 0.00 (0.00) |
| | 5 | 0.00 (0.00) | 0.00 (0.00) | 0.00 (0.00) | 0.00 (0.00) | 0.00 (0.00) | 0.00 (0.00) | 0.00 (0.00) |
| | 10 | 0.00 (0.00) | 0.00 (0.00) | 0.00 (0.00) | 0.00 (0.00) | 0.00 (0.00) | 0.00 (0.00) | 0.00 (0.00) |
| DTLZ2 | 2 | 0.61 (0.01) | **0.62** (0.00) | 0.61 (0.01) | 0.61 (0.00) | 0.60 (0.02) | 0.61 (0.01) | **0.63** (0.01) |
| | 3 | **0.78** (0.00) | 0.68 (0.02) | **0.79** (0.01) | 0.73 (0.02) | 0.77 (0.01) | **0.77** (0.01) | **0.79** (0.00) |
| | 5 | **0.94** (0.00) | 0.65 (0.02) | 0.88 (0.02) | 0.78 (0.02) | 0.84 (0.07) | **0.94** (0.00) | **0.94** (0.00) |
| | 10 | **0.84** (0.03) | 0.68 (0.01) | **0.86** (0.06) | 0.77 (0.02) | **0.84** (0.02) | **0.86** (0.02) | **0.88** (0.03) |
| DTLZ3 | 2 | 0.00 (0.00) | 0.00 (0.00) | 0.00 (0.00) | 0.00 (0.00) | 0.00 (0.00) | 0.00 (0.00) | 0.00 (0.00) |
| | 3 | 0.00 (0.00) | 0.00 (0.00) | 0.00 (0.00) | 0.00 (0.00) | 0.00 (0.00) | 0.00 (0.00) | 0.00 (0.00) |
| | 5 | 0.00 (0.00) | 0.00 (0.00) | 0.00 (0.00) | 0.00 (0.00) | 0.00 (0.00) | 0.00 (0.00) | 0.00 (0.00) |
| | 10 | 0.00 (0.00) | 0.00 (0.00) | 0.00 (0.00) | 0.00 (0.00) | 0.00 (0.00) | 0.00 (0.00) | 0.00 (0.00) |
| DTLZ4 | 2 | **0.56** (0.01) | **0.54** (0.02) | **0.55** (0.02) | **0.53** (0.02) | **0.54** (0.04) | **0.52** (0.06) | **0.57** (0.02) |
| | 3 | **0.71** (0.01) | 0.58 (0.11) | **0.62** (0.10) | 0.58 (0.04) | **0.69** (0.06) | **0.71** (0.01) | **0.72** (0.02) |
| | 5 | **0.87** (0.02) | 0.56 (0.13) | 0.50 (0.13) | 0.72 (0.09) | 0.56 (0.17) | **0.82** (0.04) | **0.87** (0.01) |
| | 10 | **0.94** (0.03) | 0.64 (0.05) | 0.60 (0.06) | 0.87 (0.04) | **0.89** (0.03) | **0.94** (0.02) | **0.89** (0.06) |
| DTLZ5 | 2 | 0.61 (0.00) | **0.62** (0.00) | 0.62 (0.01) | 0.61 (0.00) | 0.60 (0.02) | 0.61 (0.02) | **0.63** (0.00) |
| | 3 | **0.52** (0.00) | 0.42 (0.03) | **0.50** (0.01) | 0.49 (0.01) | 0.50 (0.01) | **0.51** (0.03) | **0.52** (0.00) |
| | 5 | **0.44** (0.01) | 0.31 (0.03) | 0.41 (0.01) | 0.41 (0.01) | 0.43 (0.01) | **0.44** (0.00) | **0.45** (0.00) |
| | 10 | **0.38** (0.01) | 0.29 (0.03) | 0.31 (0.03) | 0.33 (0.02) | **0.38** (0.01) | **0.38** (0.00) | **0.40** (0.00) |
| DTLZ6 | 2 | **0.56** (0.01) | 0.01 (0.02) | 0.34 (0.22) | 0.34 (0.27) | **0.49** (0.06) | 0.14 (0.10) | **0.45** (0.10) |
| | 3 | **0.42** (0.06) | 0.01 (0.01) | 0.02 (0.06) | 0.00 (0.00) | 0.22 (0.18) | 0.11 (0.08) | **0.35** (0.07) |
| | 5 | **0.33** (0.04) | 0.00 (0.00) | 0.00 (0.00) | 0.00 (0.00) | 0.00 (0.00) | 0.00 (0.00) | 0.19 (0.07) |
| | 10 | **0.17** (0.05) | 0.00 (0.00) | 0.00 (0.00) | 0.00 (0.00) | 0.00 (0.00) | 0.00 (0.00) | 0.03 (0.05) |
| DTLZ7 | 2 | 0.23 (0.01) | 0.17 (0.00) | **0.31** (0.01) | 0.18 (0.04) | 0.24 (0.06) | 0.12 (0.02) | 0.25 (0.03) |
| | 3 | 0.17 (0.02) | 0.14 (0.02) | **0.31** (0.04) | 0.14 (0.02) | 0.20 (0.05) | 0.11 (0.05) | 0.21 (0.04) |
| | 5 | 0.12 (0.03) | 0.00 (0.00) | **0.19** (0.03) | 0.03 (0.03) | 0.11 (0.05) | 0.06 (0.02) | 0.13 (0.03) |
| | 10 | **0.07** (0.02) | 0.00 (0.00) | 0.03 (0.04) | 0.01 (0.02) | 0.00 (0.00) | 0.01 (0.01) | 0.02 (0.03) |

Table 3: Mean hypervolume values and standard deviation (in parentheses) for DTLZ problems. The values statistically similar to the best one are in bold, the best value is encircled the worst value is underlined

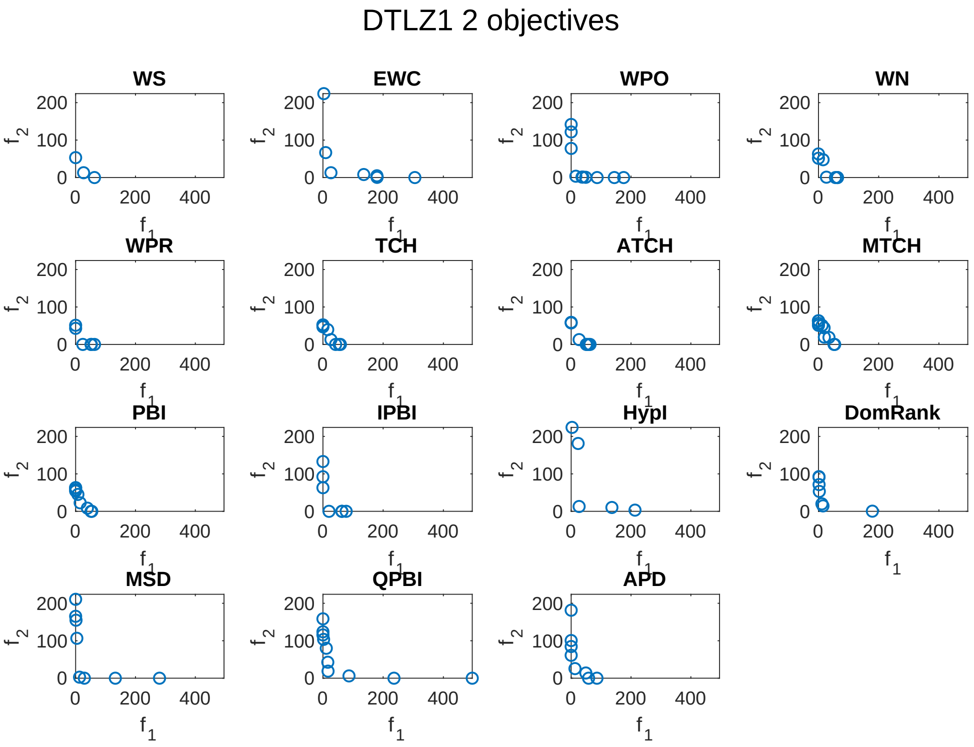
DTLZ1 2 objectives
WS
EWC
WPO
WN
WPR
TCH
ATCH
MTCH
PBI
IPBI
HypI
DomRank
MSD
QPBI
APD
$f_1$
$f_2$

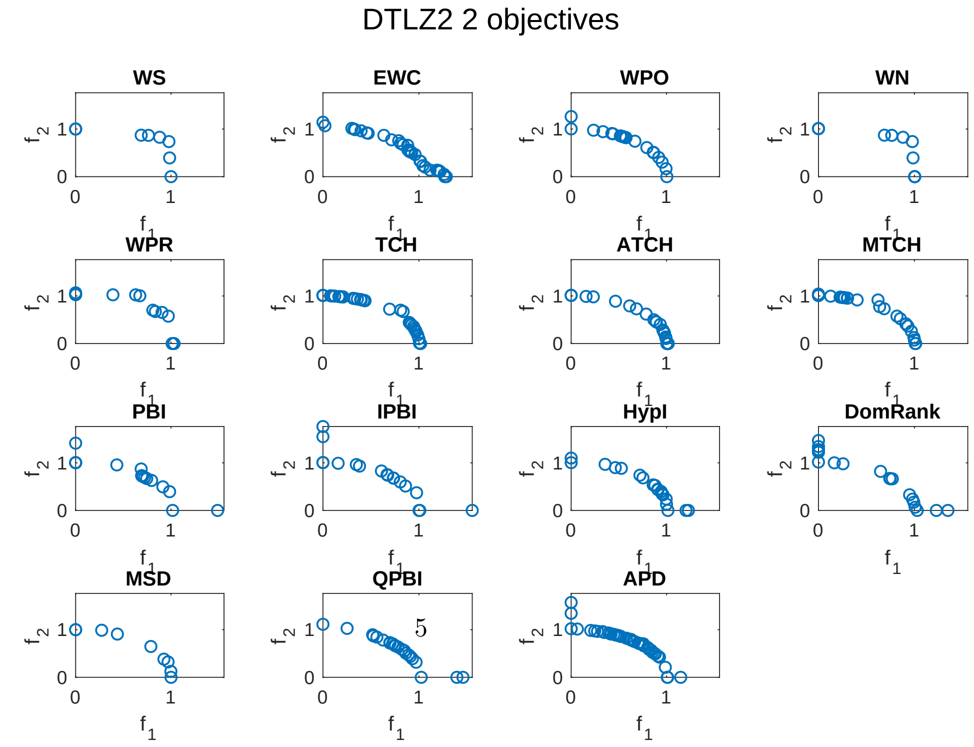
DTLZ2 2 objectives
WS
EWC
WPO
WN
WPR
TCH
ATCH
MTCH
PBI
IPBI
HypI
DomRank
MSD
QPBI
APD
$f_1$
$f_2$



Figure 1

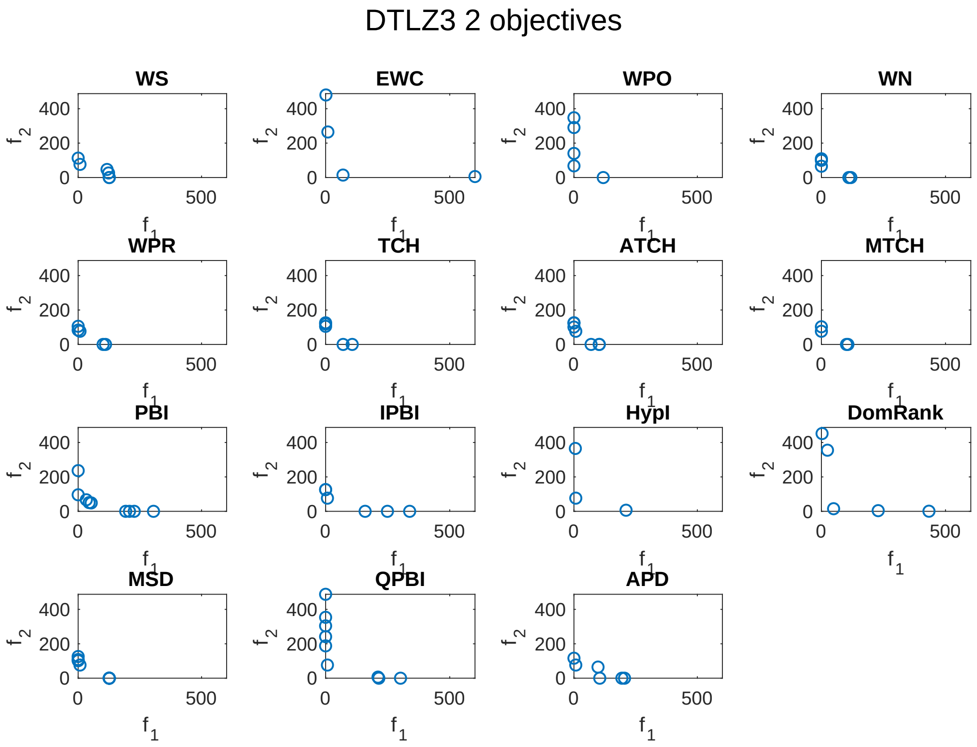
DTLZ3 2 objectives
WS
EWC
WPO
WN
WPR
TCH
ATCH
MTCH
PBI
IPBI
HypI
DomRank
MSD
QPBI
APD
f 1
f 2
0
200
400
500

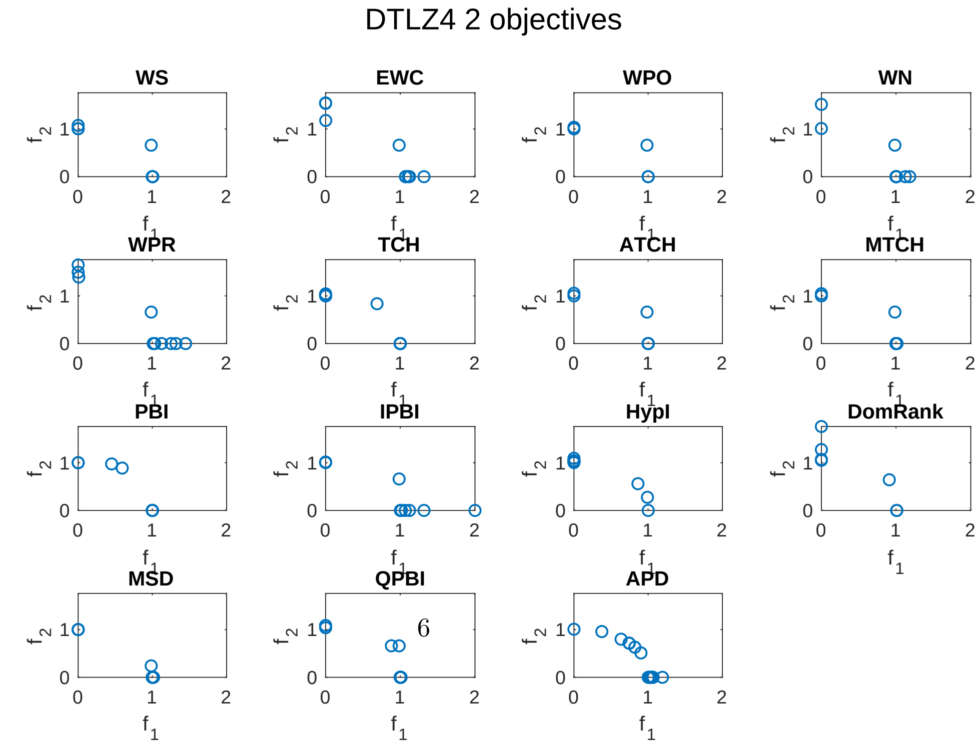
DTLZ4 2 objectives
WS
EWC
WPO
WN
WPR
TCH
ATCH
MTCH
PBI
IPBI
HypI
DomRank
MSD
QPBI
APD
f 1
f 2
0
1
2



Figure 2

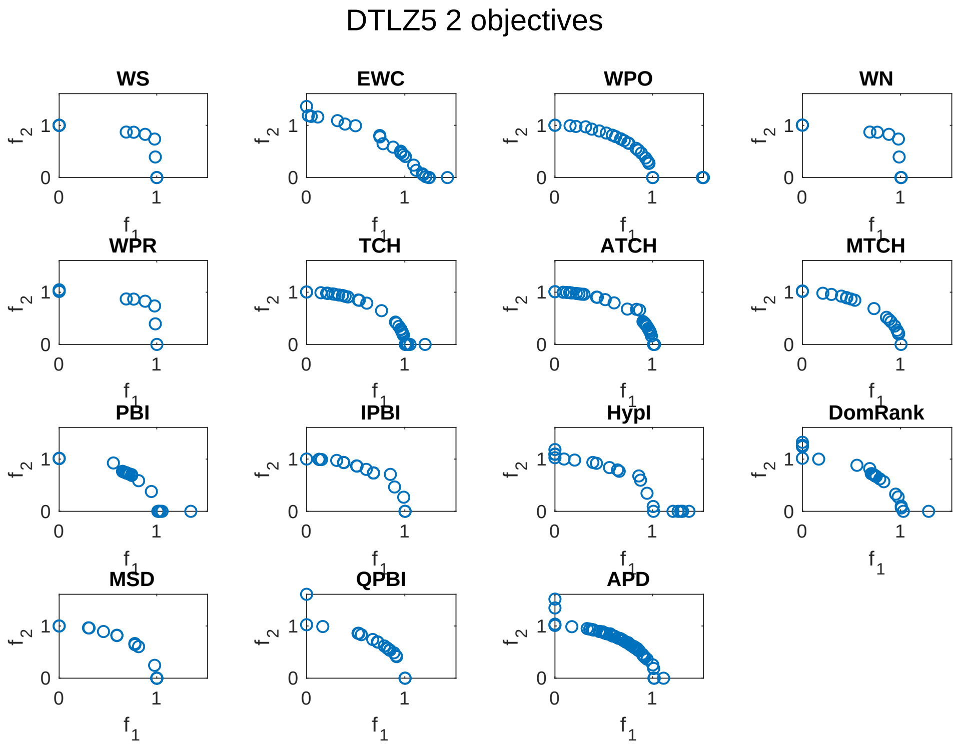
DTLZ5 2 objectives
WS
EWC
WPO
WN
WPR
TCH
ATCH
MTCH
PBI
IPBI
HypI
DomRank
MSD
QPBI
APD
f 1
f 2

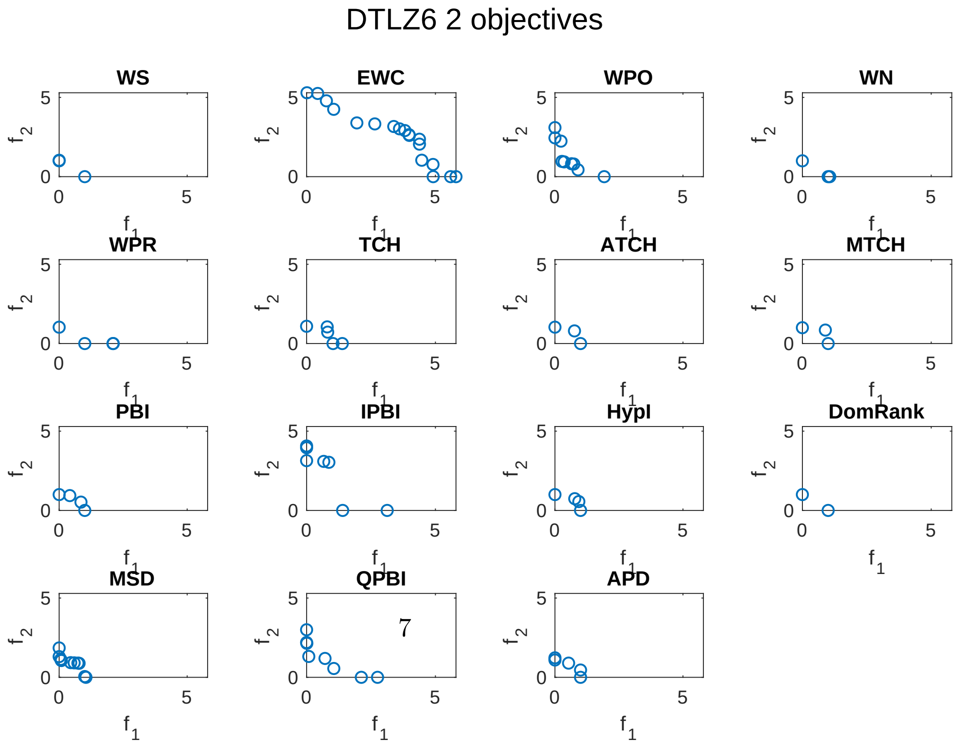
DTLZ6 2 objectives
WS
EWC
WPO
WN
WPR
TCH
ATCH
MTCH
PBI
IPBI
HypI
DomRank
MSD
QPBI
APD
f 1
f 2

Figure 3

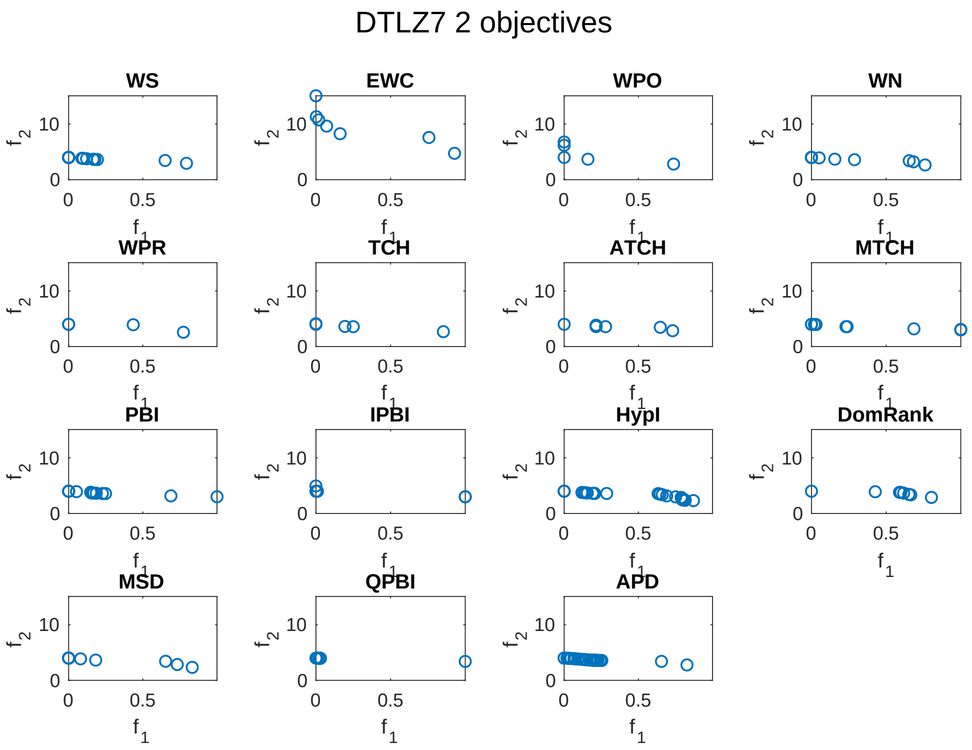
DTLZ7 2 objectives
WS
EWC
WPO
WN
WPR
TCH
ATCH
MTCH
PBI
IPBI
HypI
DomRank
MSD
QPBI
APD
f 2
f 1
0
10
0.5

Figure 4

### 3.2 Three objectives DTLZ problems

The scatter plots of the approximated Pareto fronts of three objectives DTLZ problems are shown in Figures 5-8.

### 3.3 Five objectives DTLZ problems

The arallel coordinate plots of the approximated Pareto fronts of five objectives DTLZ problems are shown in Figures 9-12.

### 3.4 Ten objectives DTLZ problems

The parallel coordinate plots of the approximated Pareto fronts of ten objectives DTLZ problems are shown in Figures 13-16.

## 4 Fitness landscapes

In this section, we show the scalarizing function values (notated by g) on different problems. Note that for a given number of objective value, we used the same training and testing data sets and also used the same weight vector when building surrogates. These results clearly showed the sensitivity of different functions to the number of objectives, which is also explained in details in the main manuscript.

### 4.1 Two Objectives DTLZ problems

The fitness landscapes for two objecives problems are shown in Figures 17-23.

### 4.2 Three Objectives DTLZ problems

The fitness landscapes of three objectives problems are shown in Figures 24-30.

### 4.3 Five objectives DTLZ problems

The fitness landscapes of five objectives problems are shown in Figures 31-37.

### 4.4 Ten Objectives DTLZ problems

The fitness landscapes of five objectives problems are shown in Figures 38-44.

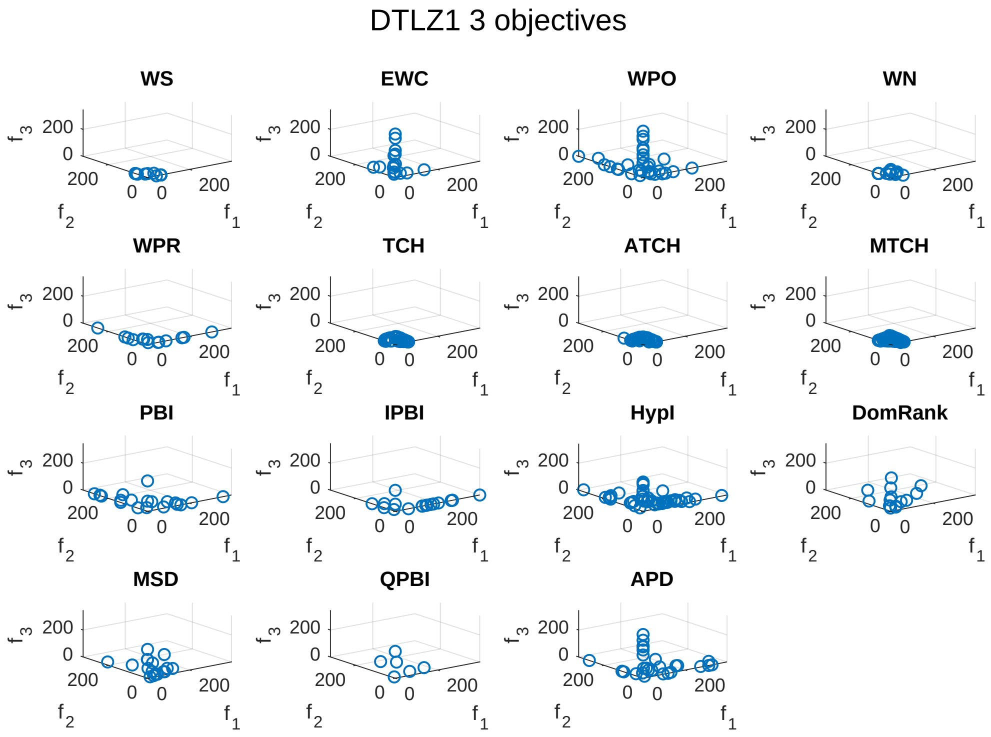
DTLZ1 3 objectives
WS
EWC
WPO
WN
WPR
TCH
ATCH
MTCH
PBI
IPBI
HypI
DomRank
MSD
QPBI
APD
f1
f2
f3
200
0

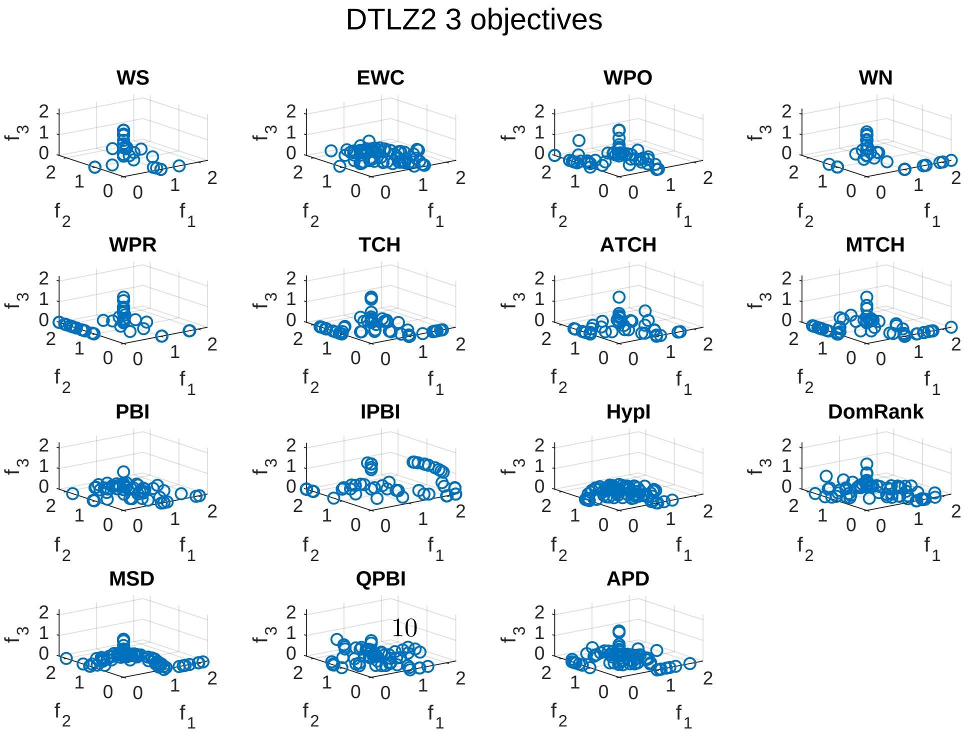
DTLZ2 3 objectives
WS
EWC
WPO
WN
WPR
TCH
ATCH
MTCH
PBI
IPBI
HypI
DomRank
MSD
QPBI
APD
f1
f2
f3
0
1
2



Figure 5

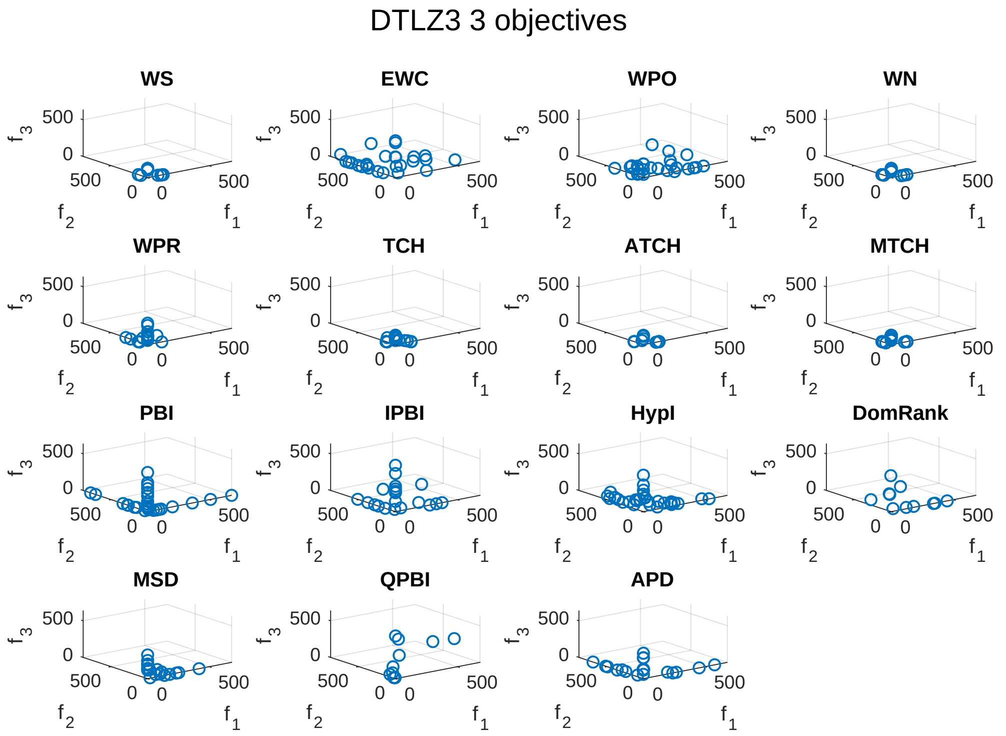
DTLZ3 3 objectives
WS
EWC
WPO
WN
WPR
TCH
ATCH
MTCH
PBI
IPBI
HypI
DomRank
MSD
QPBI
APD

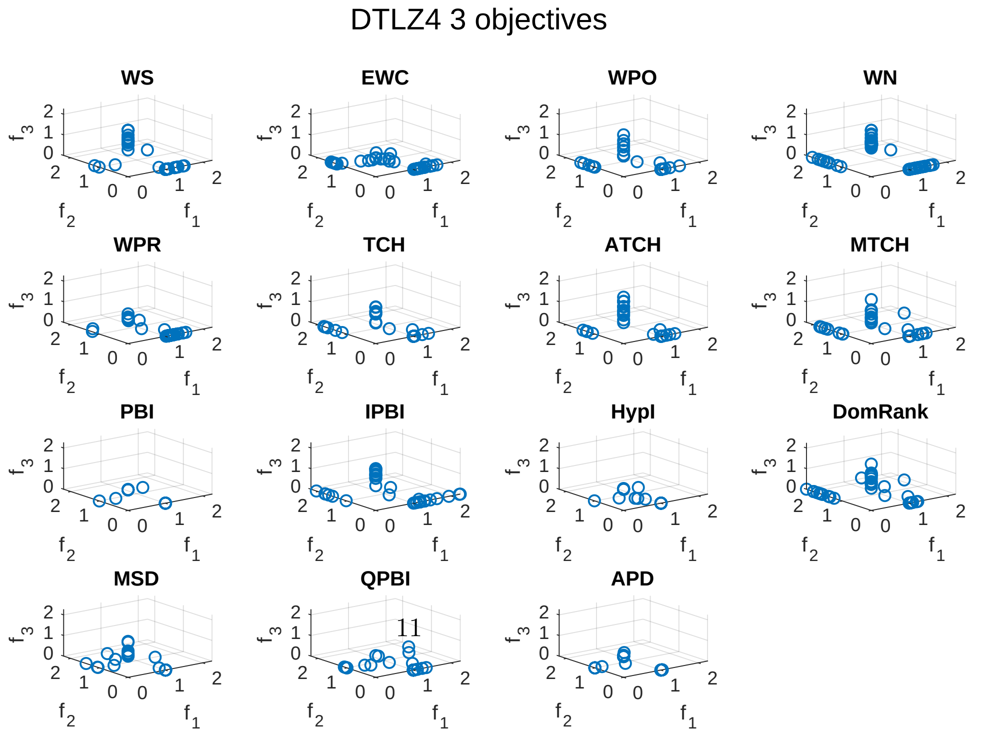
DTLZ4 3 objectives
WS
EWC
WPO
WN
WPR
TCH
ATCH
MTCH
PBI
IPBI
HypI
DomRank
MSD
QPBI
APD



Figure 6

DTLZ5 3 objectives

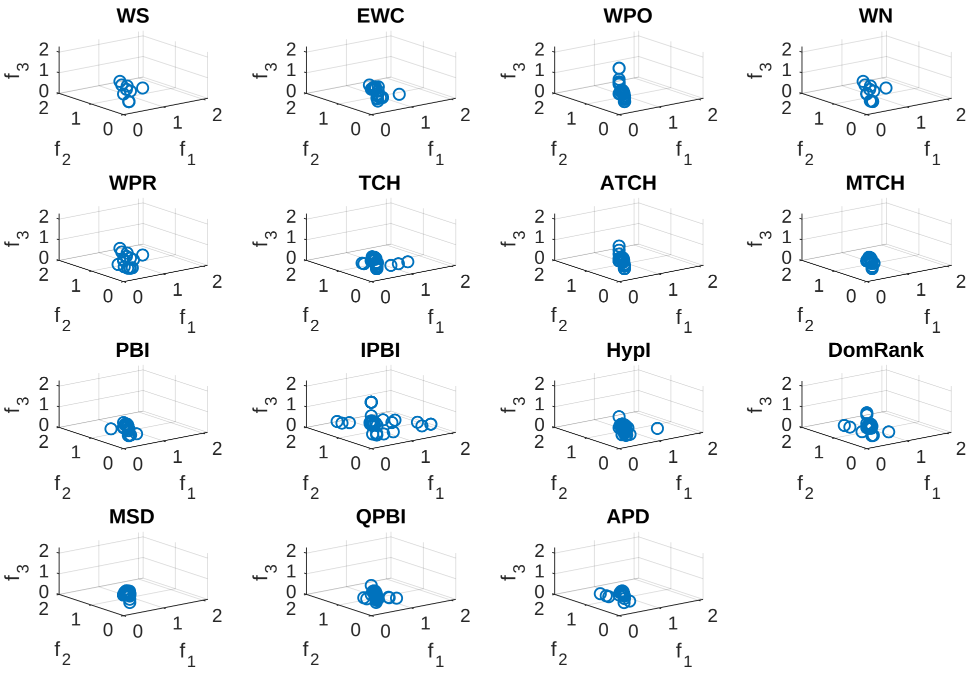


DTLZ6 3 objectives

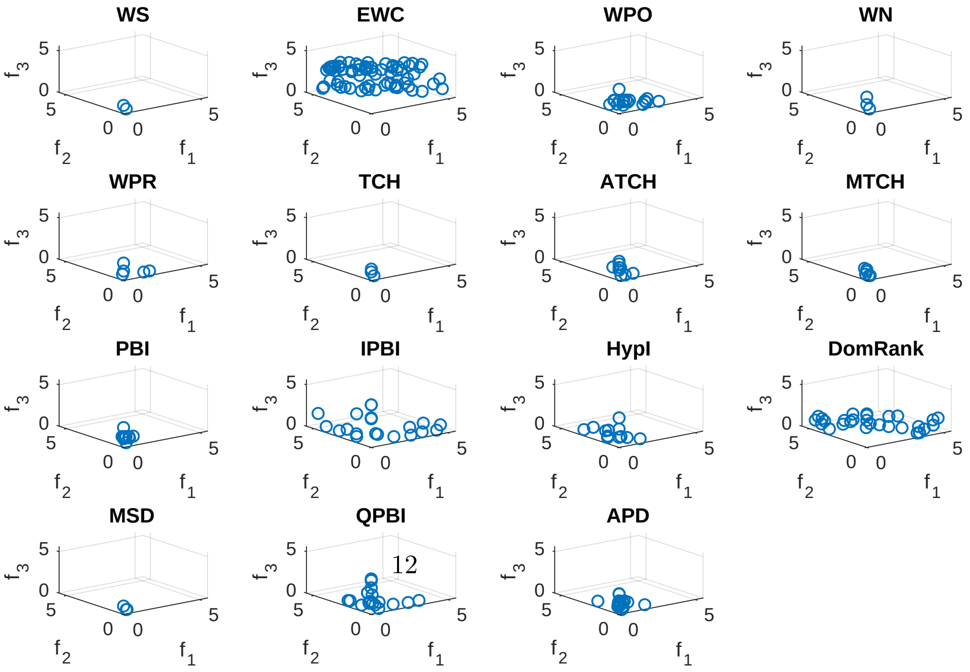


Figure 7

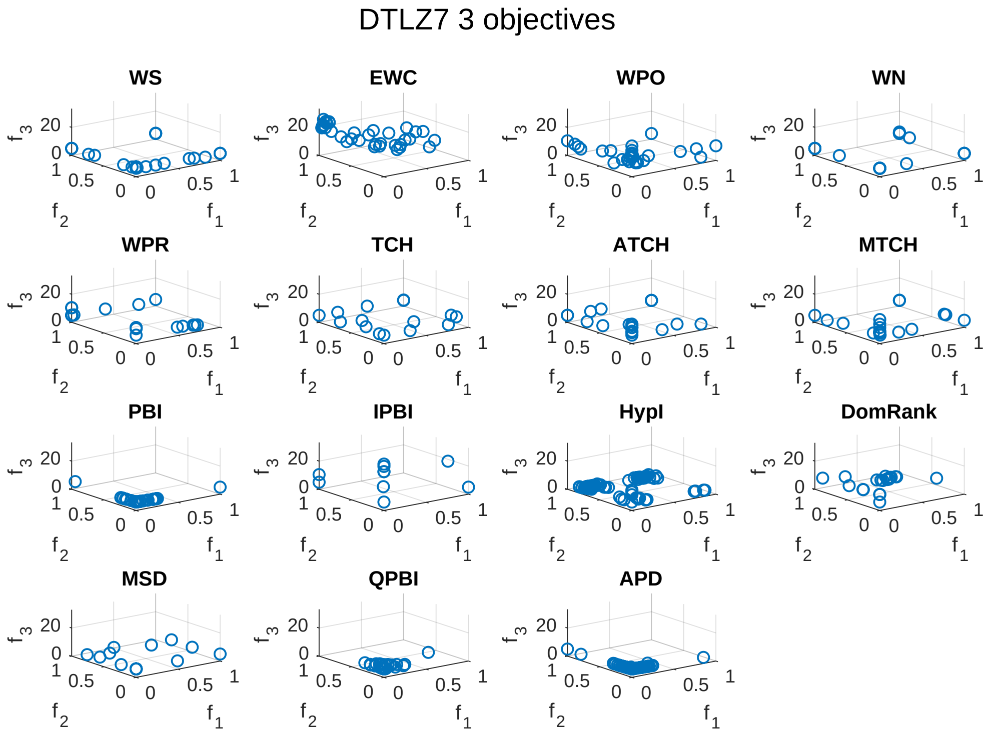
DTLZ7 3 objectives
WS
EWC
WPO
WN
WPR
TCH
ATCH
MTCH
PBI
IPBI
HypI
DomRank
MSD
QPBI
APD

Figure 8

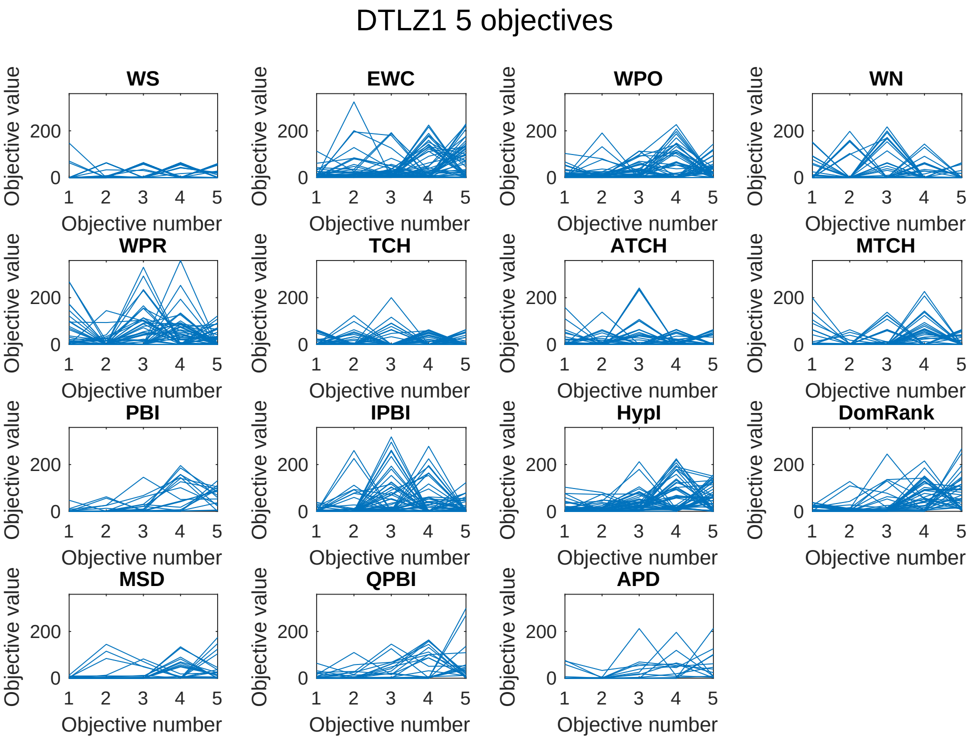
DTLZ1 5 objectives
WS
EWC
WPO
WN
WPR
TCH
ATCH
MTCH
PBI
IPBI
HypI
DomRank
MSD
QPBI
APD
Objective value
Objective number

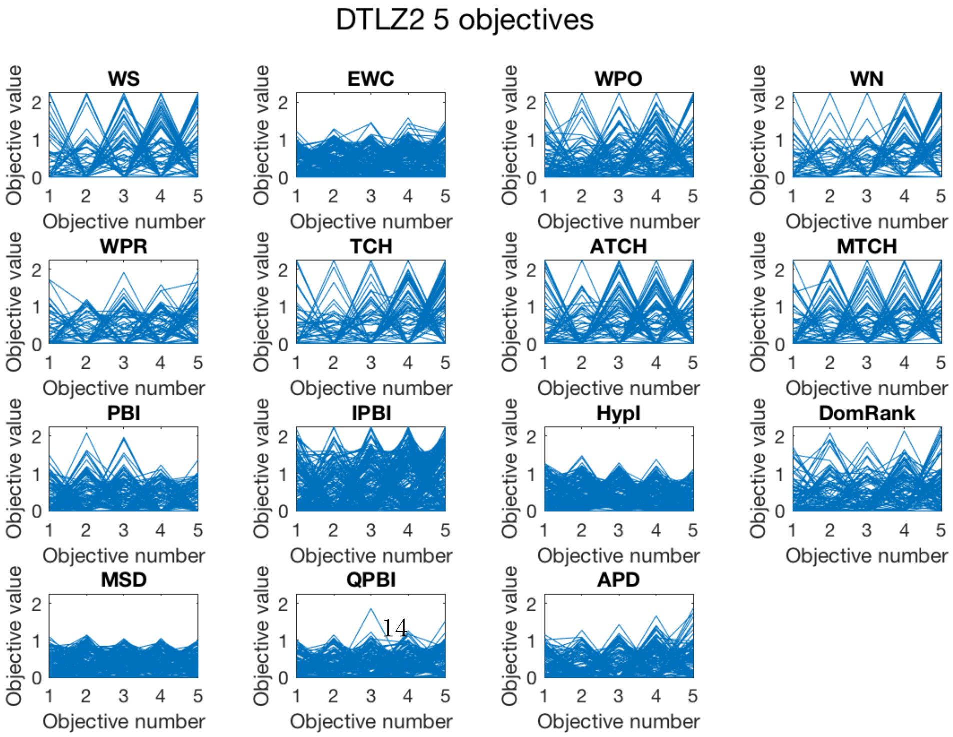
DTLZ2 5 objectives
WS
EWC
WPO
WN
WPR
TCH
ATCH
MTCH
PBI
IPBI
HypI
DomRank
MSD
QPBI
APD
Objective value
Objective number



Figure 9

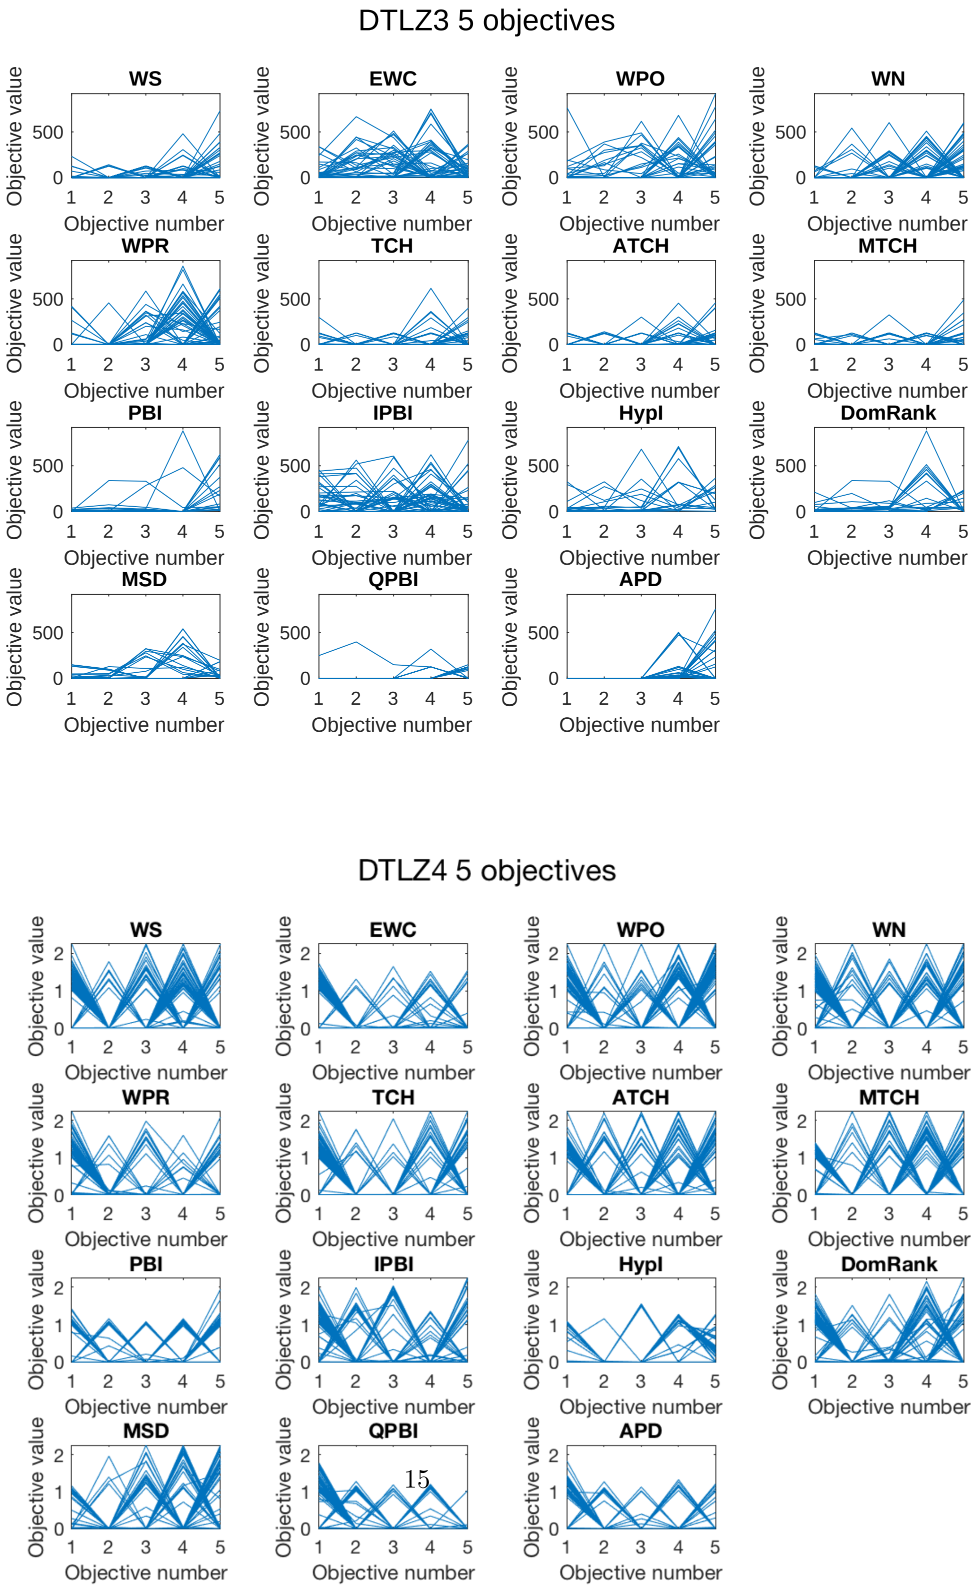
DTLZ3 5 objectives
WS
EWC
WPO
WN
WPR
TCH
ATCH
MTCH
PBI
IPBI
HypI
DomRank
MSD
QPBI
APD
Objective value
Objective number
DTLZ4 5 objectives
WS
EWC
WPO
WN
WPR
TCH
ATCH
MTCH
PBI
IPBI
HypI
DomRank
MSD
QPBI
APD
Objective value
Objective number



Figure 10

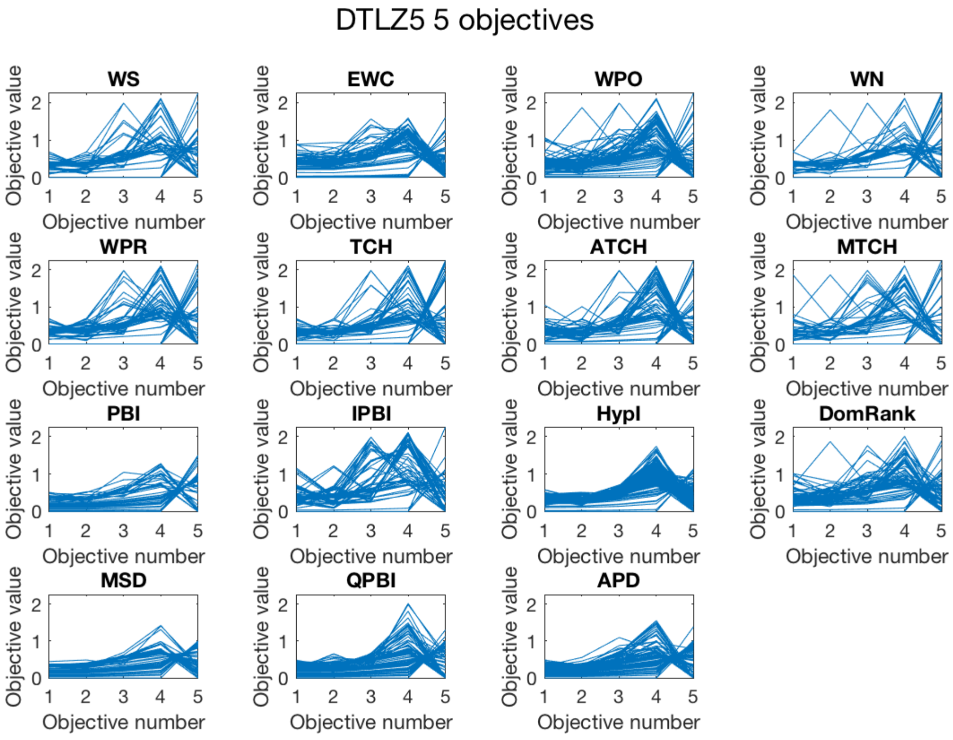
DTLZ5 5 objectives
WS
EWC
WPO
WN
WPR
TCH
ATCH
MTCH
PBI
IPBI
HypI
DomRank
MSD
QPBI
APD
Objective value
Objective number

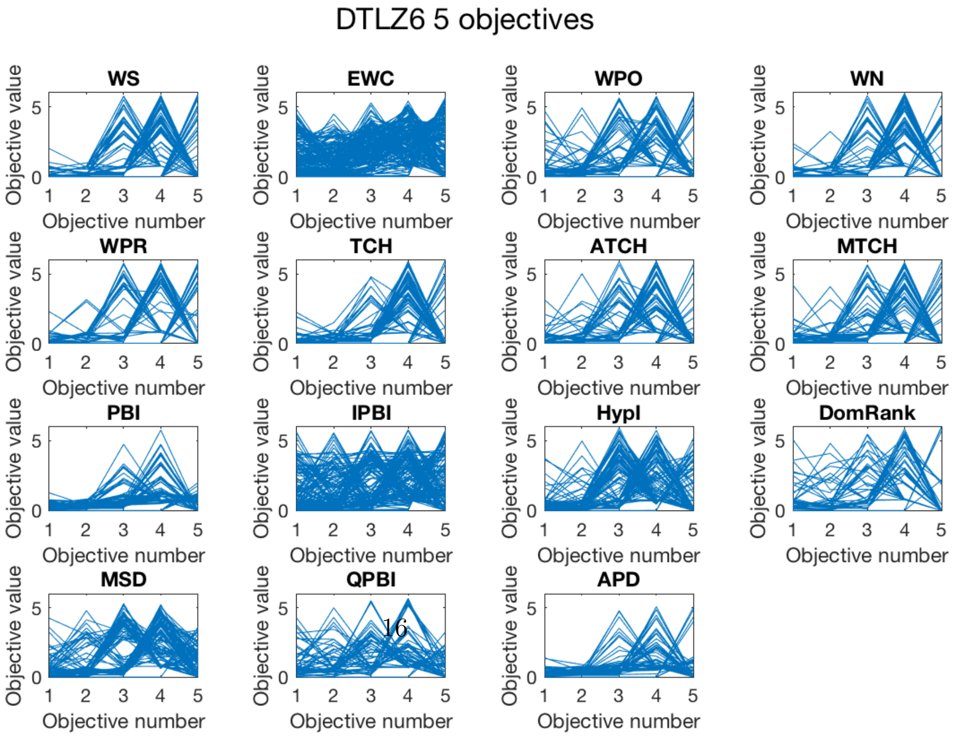
DTLZ6 5 objectives
WS
EWC
WPO
WN
WPR
TCH
ATCH
MTCH
PBI
IPBI
HypI
DomRank
MSD
QPBI
APD
Objective value
Objective number



Figure 11

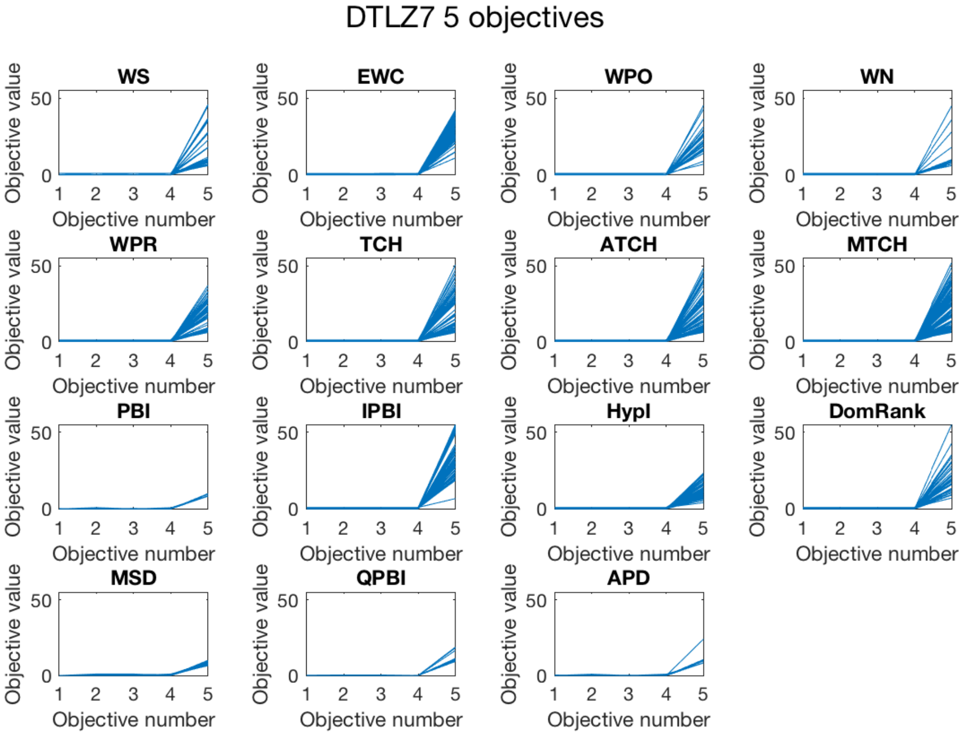
DTLZ7 5 objectives
WS
EWC
WPO
WN
WPR
TCH
ATCH
MTCH
PBI
IPBI
HypI
DomRank
MSD
QPBI
APD
Objective value
Objective number
50
0
1
2
3
4
5

Figure 12

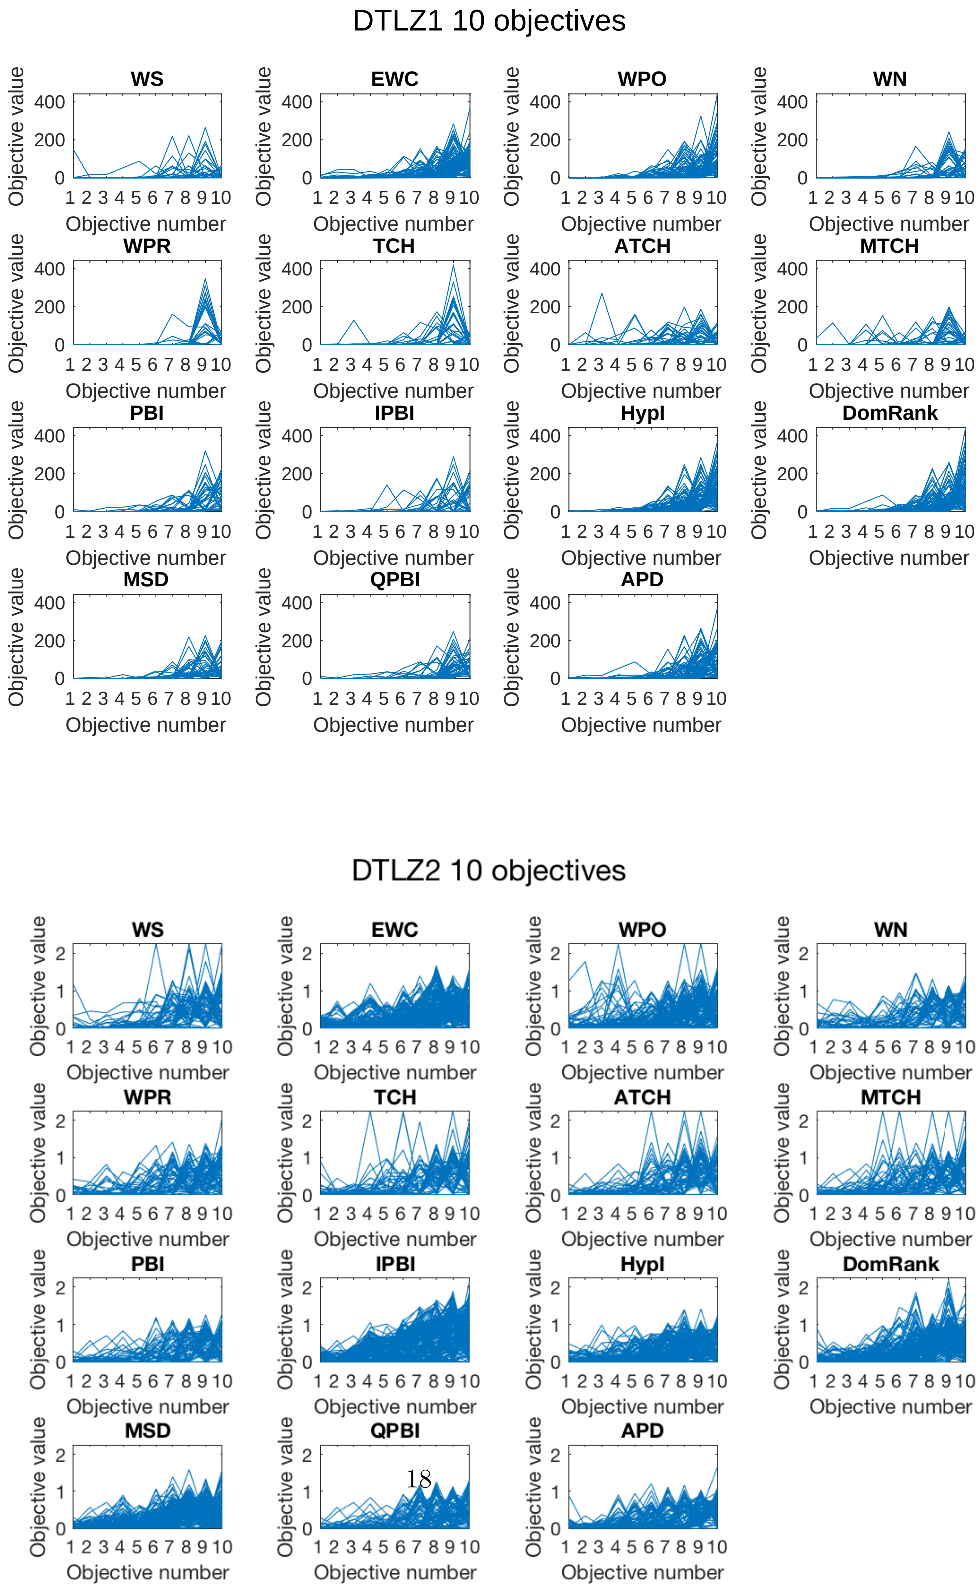
DTLZ1 10 objectives
WS
EWC
WPO
WN
WPR
TCH
ATCH
MTCH
PBI
IPBI
HypI
DomRank
MSD
QPBI
APD
Objective value
Objective number
DTLZ2 10 objectives
WS
EWC
WPO
WN
WPR
TCH
ATCH
MTCH
PBI
IPBI
HypI
DomRank
MSD
QPBI
APD
Objective value
Objective number



Figure 13

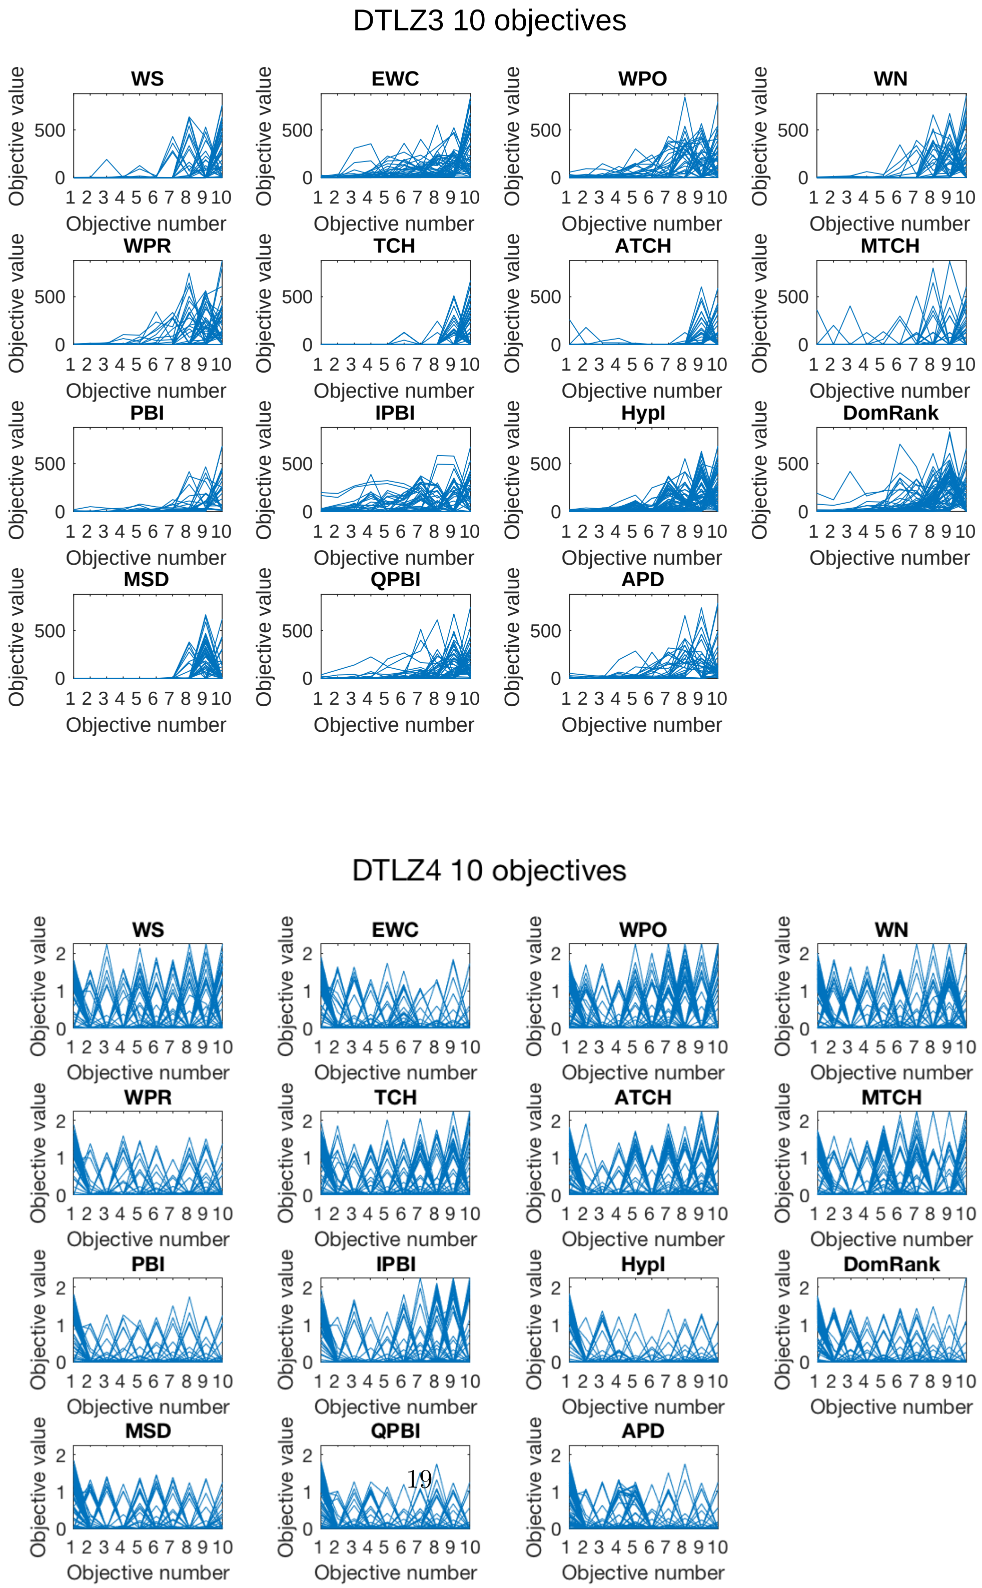
DTLZ3 10 objectives
WS
EWC
WPO
WN
WPR
TCH
ATCH
MTCH
PBI
IPBI
HypI
DomRank
MSD
QPBI
APD
Objective value
Objective number
DTLZ4 10 objectives
WS
EWC
WPO
WN
WPR
TCH
ATCH
MTCH
PBI
IPBI
HypI
DomRank
MSD
QPBI
APD
Objective value
Objective number



Figure 14

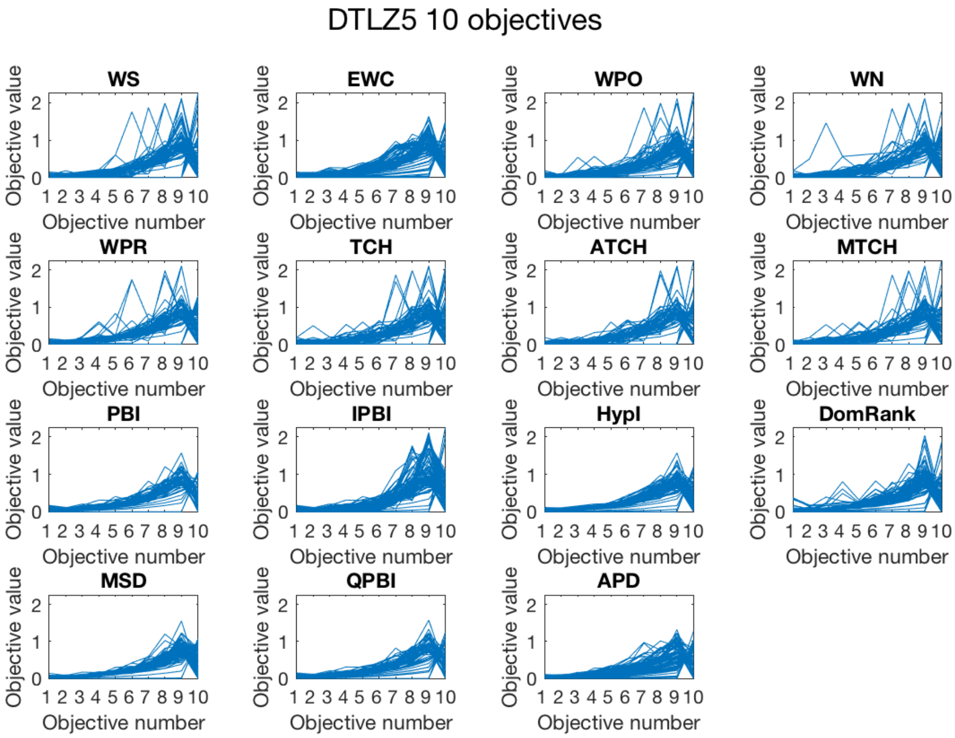
DTLZ5 10 objectives
WS
EWC
WPO
WN
WPR
TCH
ATCH
MTCH
PBI
IPBI
HypI
DomRank
MSD
QPBI
APD
Objective value
Objective number
0
1
2
1 2 3 4 5 6 7 8 9 10

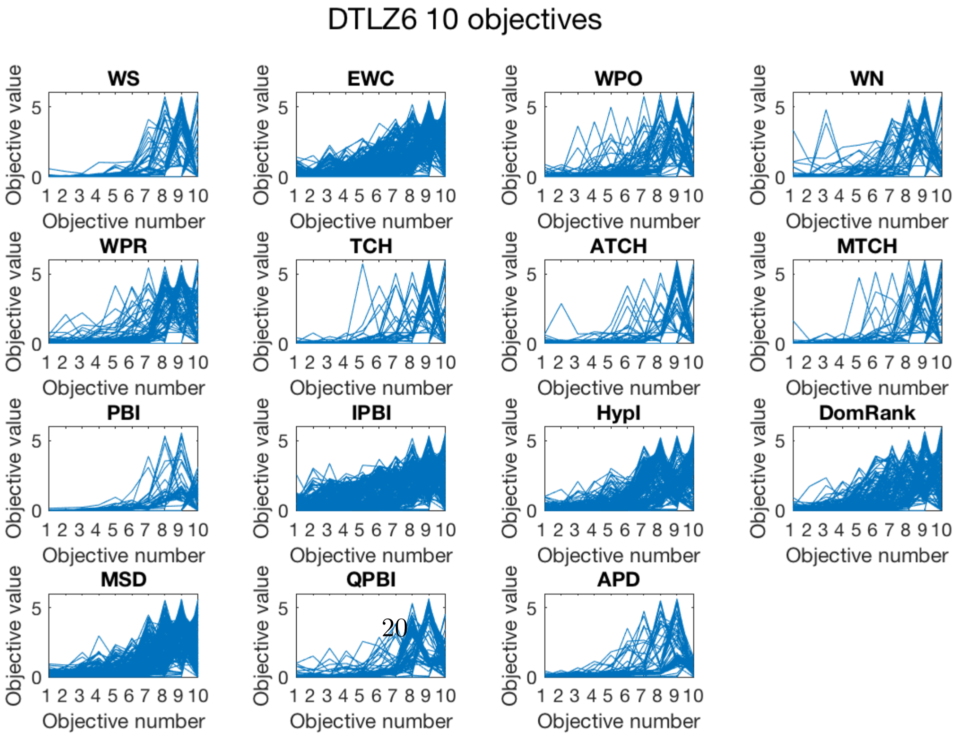
DTLZ6 10 objectives
WS
EWC
WPO
WN
WPR
TCH
ATCH
MTCH
PBI
IPBI
HypI
DomRank
MSD
QPBI
APD
Objective value
Objective number
0
5
1 2 3 4 5 6 7 8 9 10



Figure 15

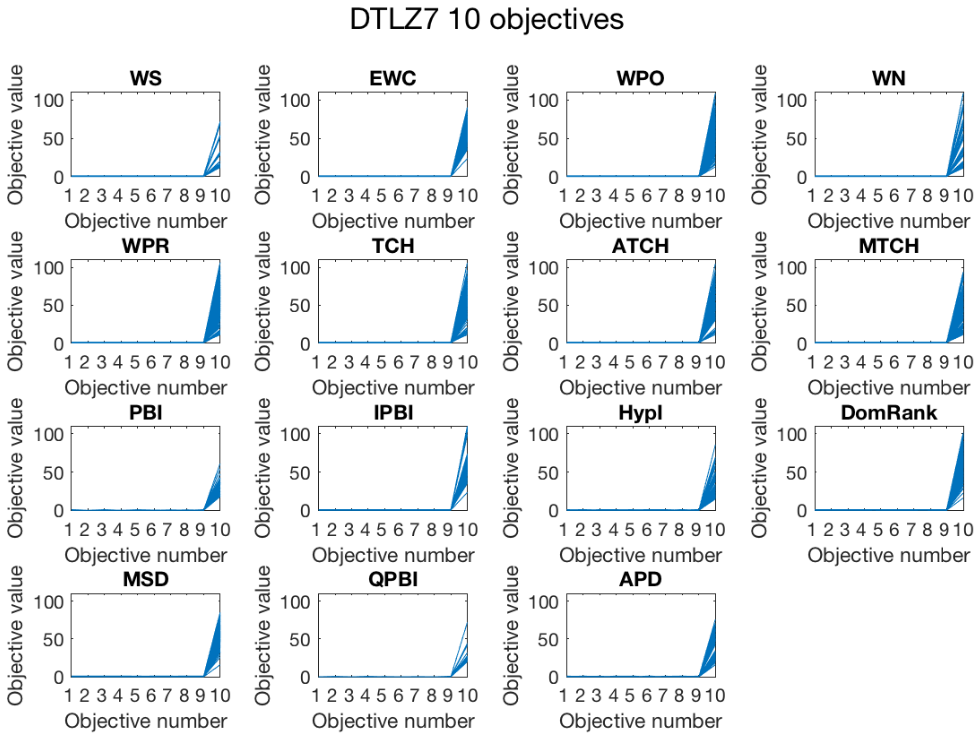
DTLZ7 10 objectives
WS
EWC
WPO
WN
WPR
TCH
ATCH
MTCH
PBI
IPBI
HypI
DomRank
MSD
QPBI
APD
Objective value
Objective number
0
50
100
1 2 3 4 5 6 7 8 9 10

Figure 16

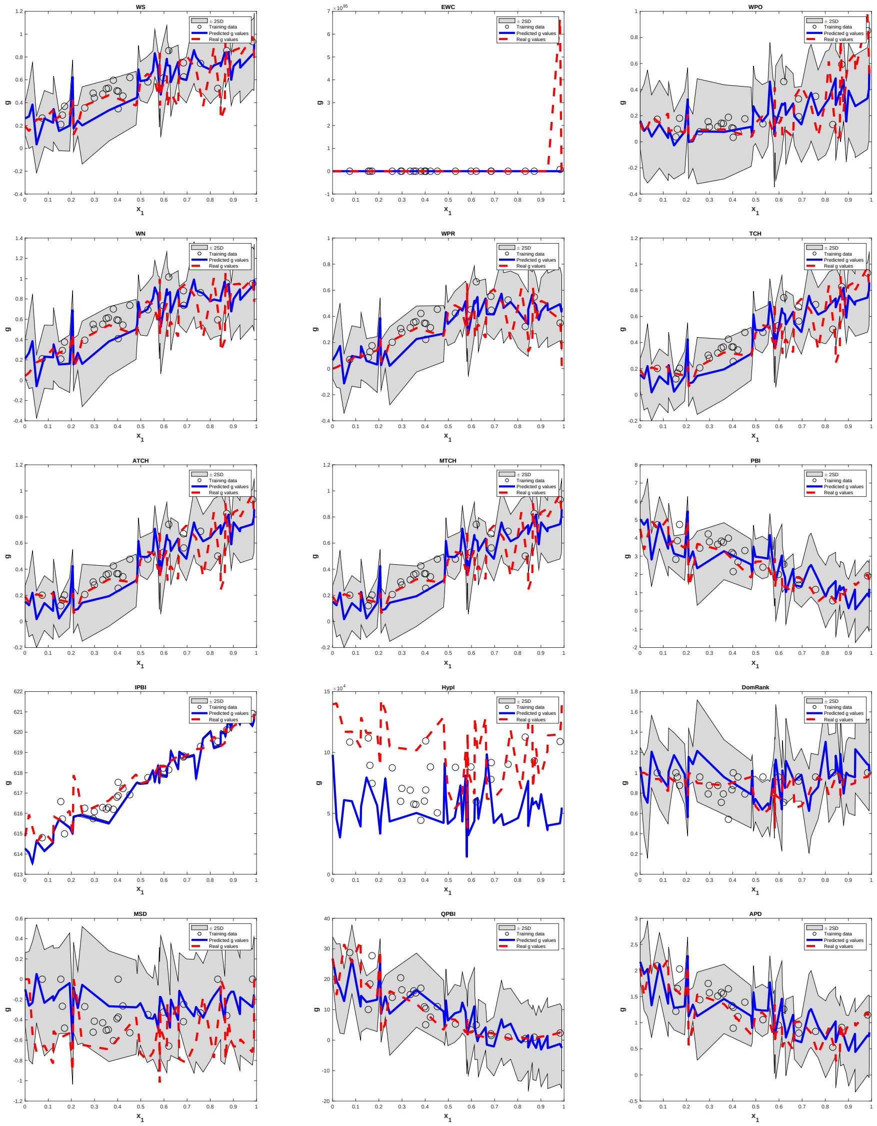


Figure 17: Scalarizing function values (notated by g) with one decision variable value for DTLZ1 two objectives, ±2SD represents the predicted g values with ± 2 standard deviations or uncertainty of the predicted values

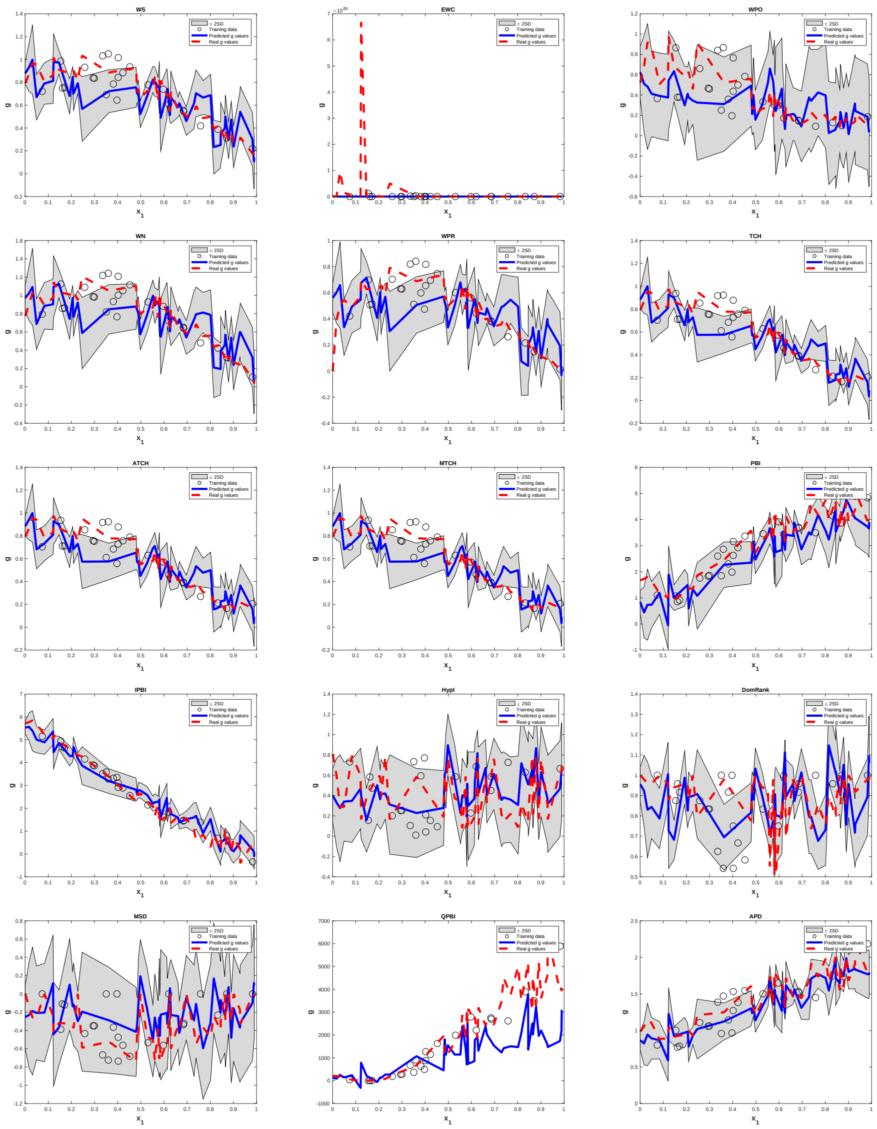


Figure 18: Scalarizing function values (notated by g) with one decision variable value for DTLZ2 two objectives, ±2SD represents the predicted g values with ± 2 standard deviations or uncertainty of the predicted values

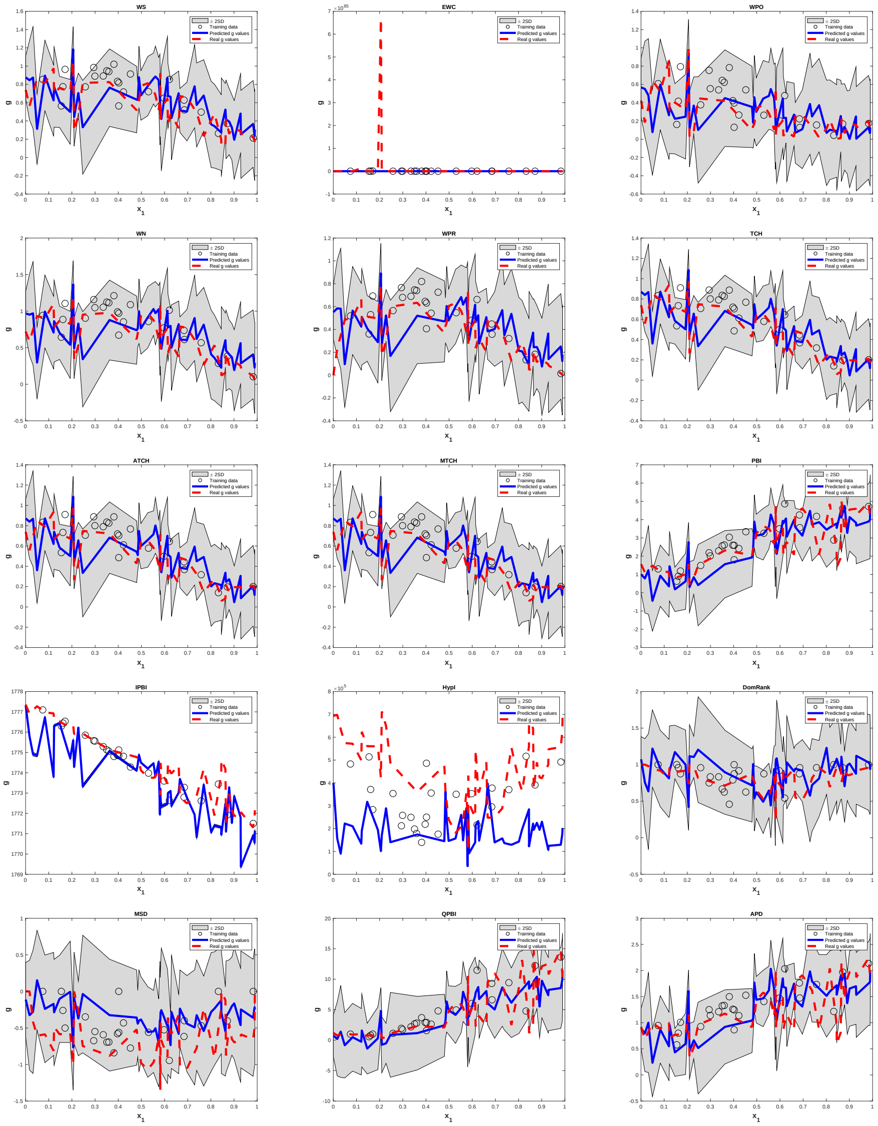

Figure 19: Scalarizing function values (notated by g) with one decision variable value for DTLZ3 two objectives, ±2SD represents the predicted g values with ± 2 standard deviations or uncertainty of the predicted values

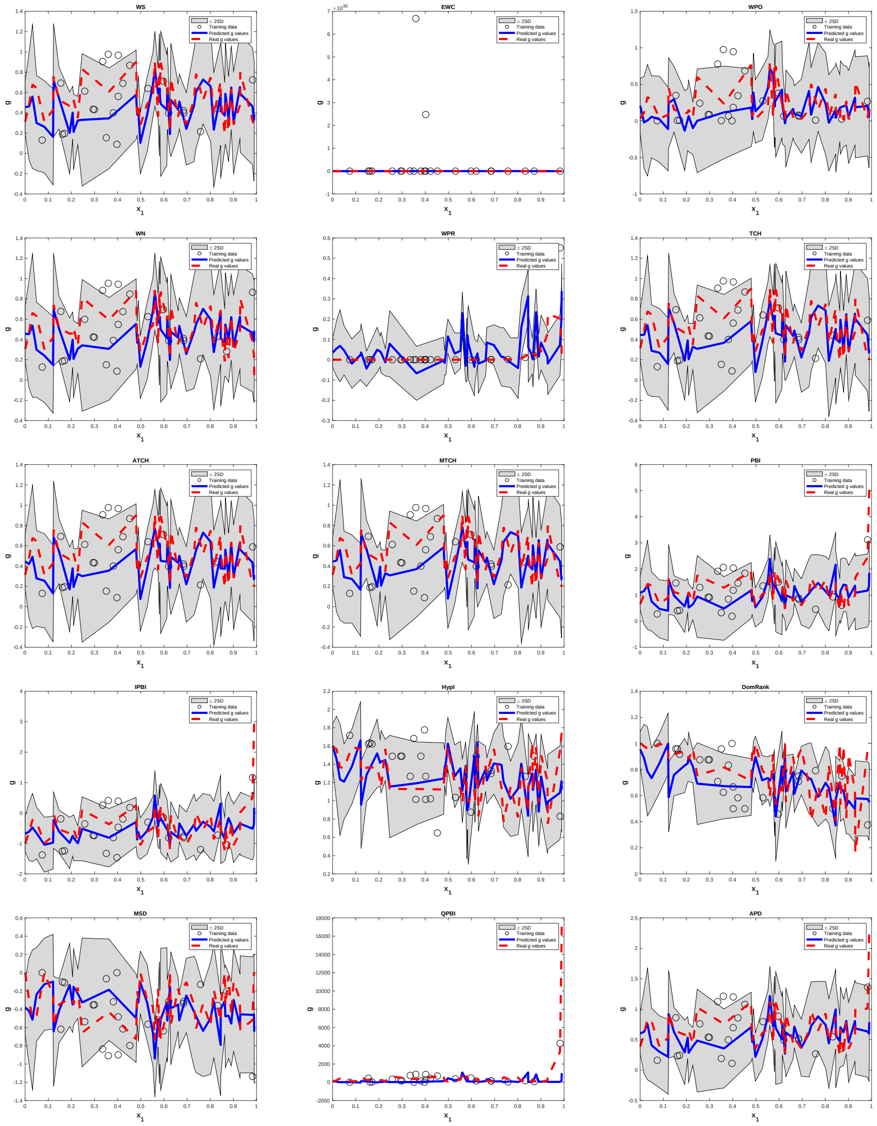


Figure 20: Scalarizing function values (notated by g) with one decision variable value for DTLZ4 two objectives, ±2SD represents the predicted g values with ± 2 standard deviations or uncertainty of the predicted values

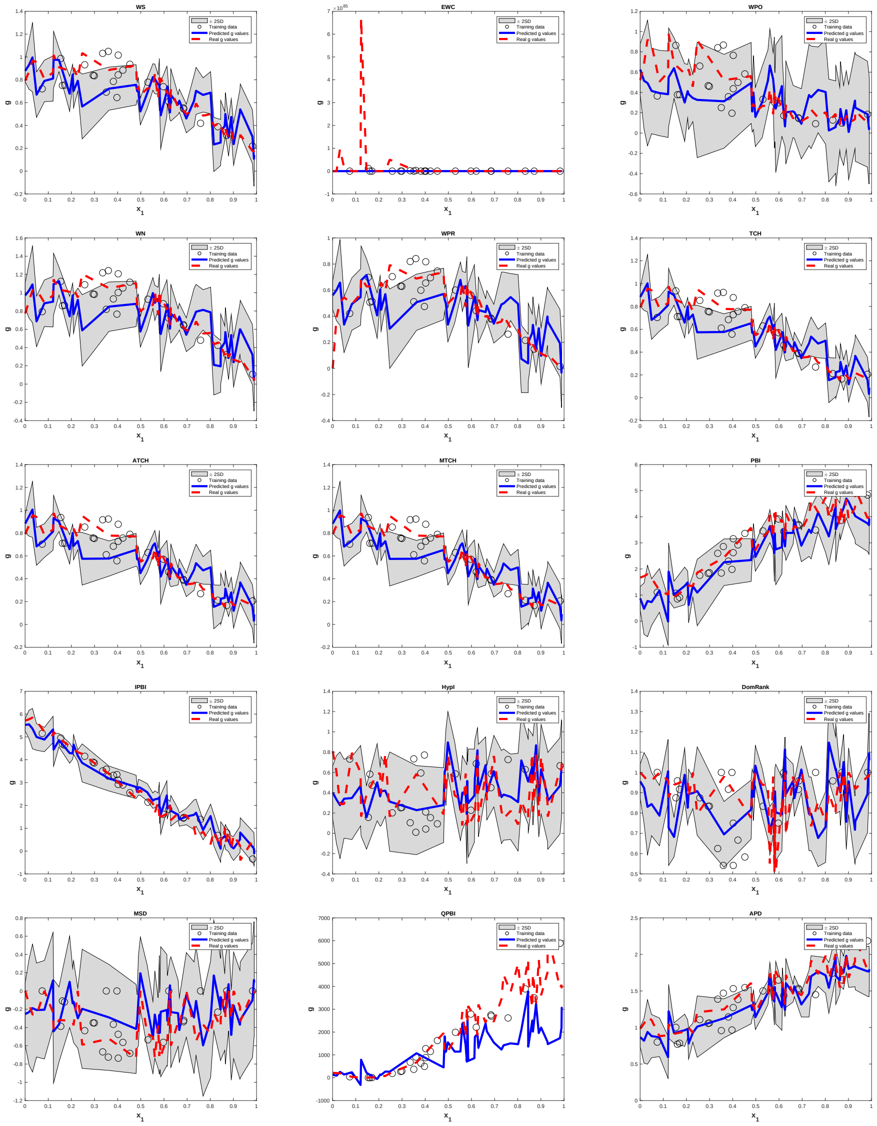

Figure 21: Scalarizing function values (notated by g) with one decision variable value for DTLZ5 two objectives, ±2SD represents the predicted g values with ± 2 standard deviations or uncertainty of the predicted values

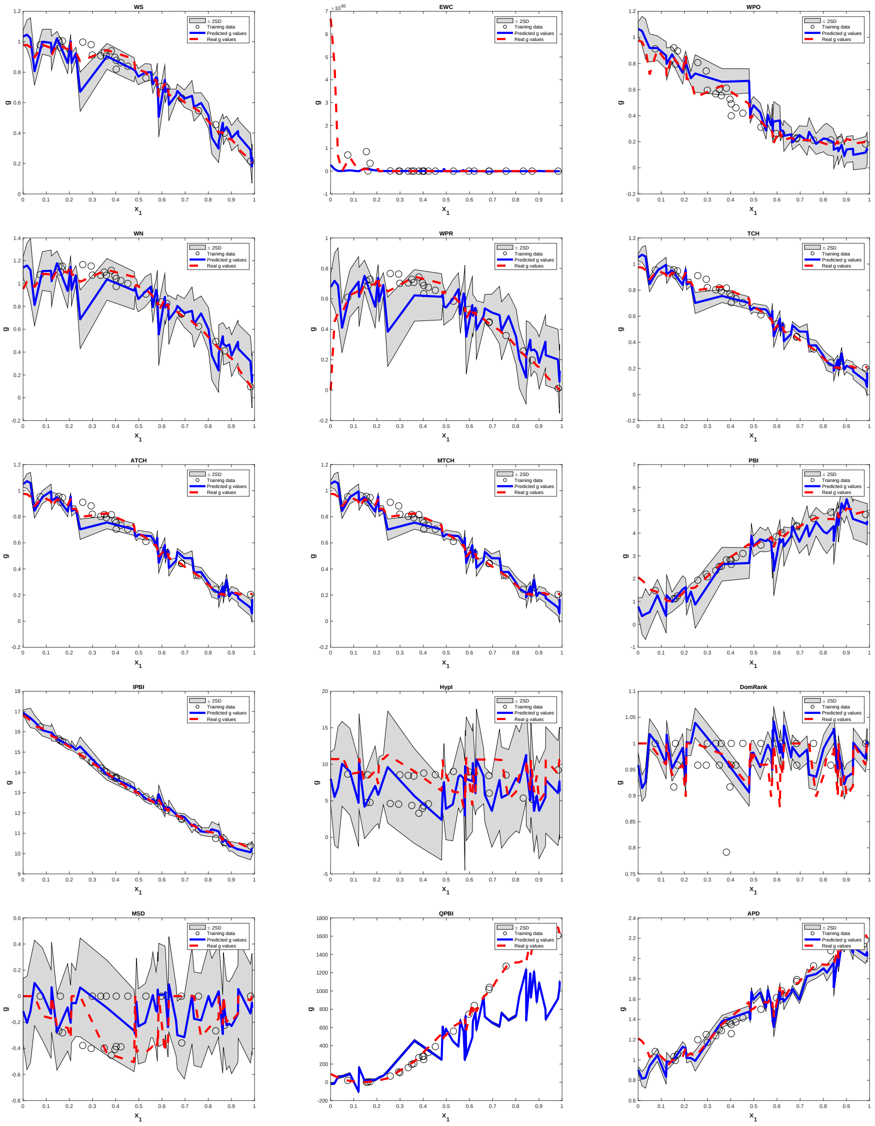


Figure 22: Scalarizing function values (notated by g) with one decision variable value for DTLZ6 two objectives, ±2SD represents the predicted g values with ± 2 standard deviations or uncertainty of the predicted values

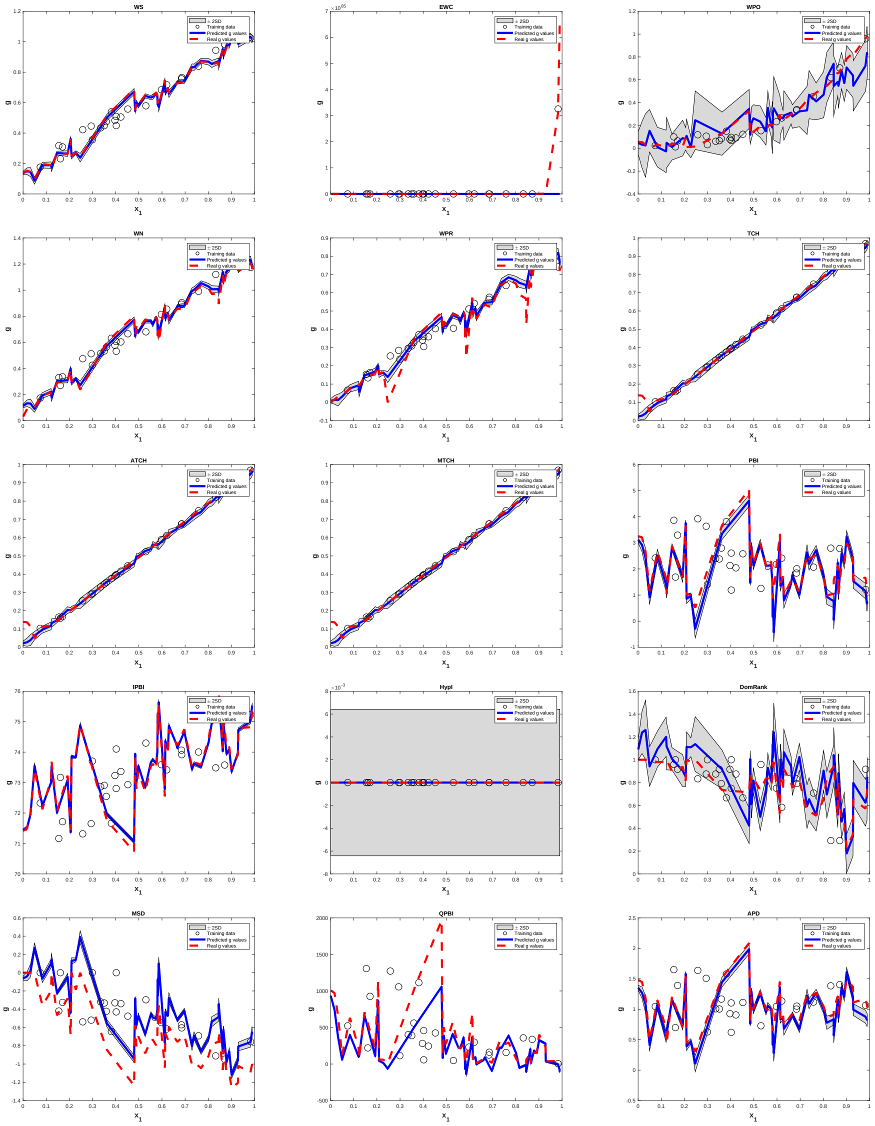


Figure 23: Scalarizing function values (notated by g) with one decision variable value for DTLZ7 two objectives, $\pm$2SD represents the predicted g values with $\pm$ 2 standard deviations or uncertainty of the predicted values

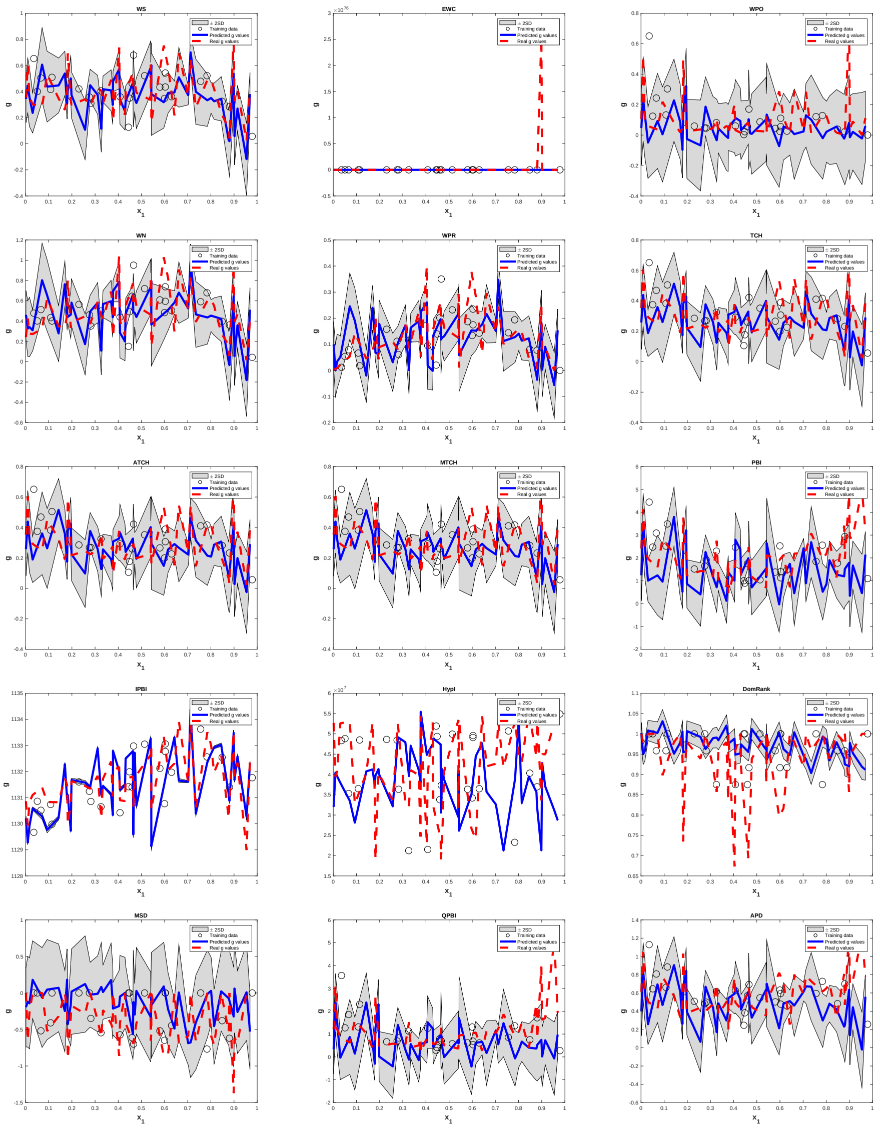


Figure 24: Scalarizing function values (notated by g) with one decision variable value for DTLZ1 three objectives, ±2SD represents the predicted g values with ± 2 standard deviations or uncertainty of the predicted values

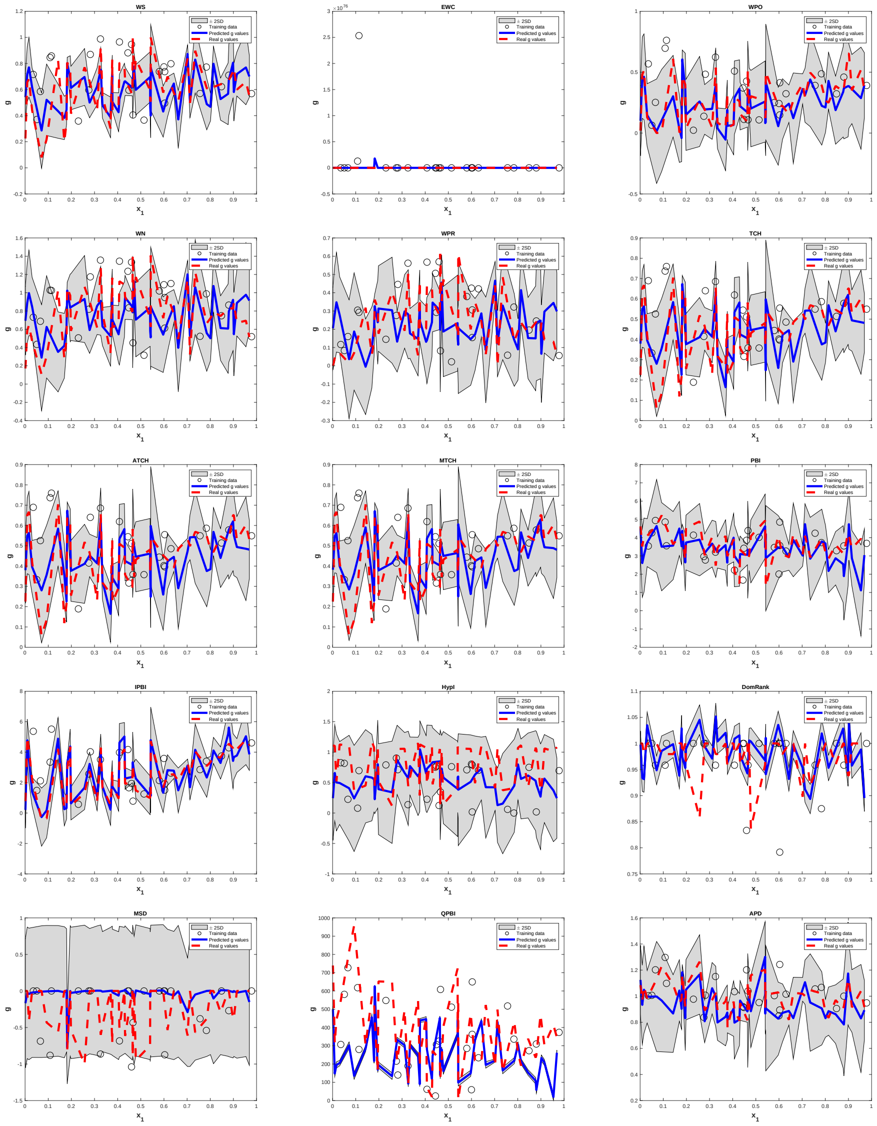

Figure 25: Scalarizing function values (notated by g) with one decision variable value for DTLZ2 three objectives, ±2SD represents the predicted g values with ± 2 standard deviations or uncertainty of the predicted values

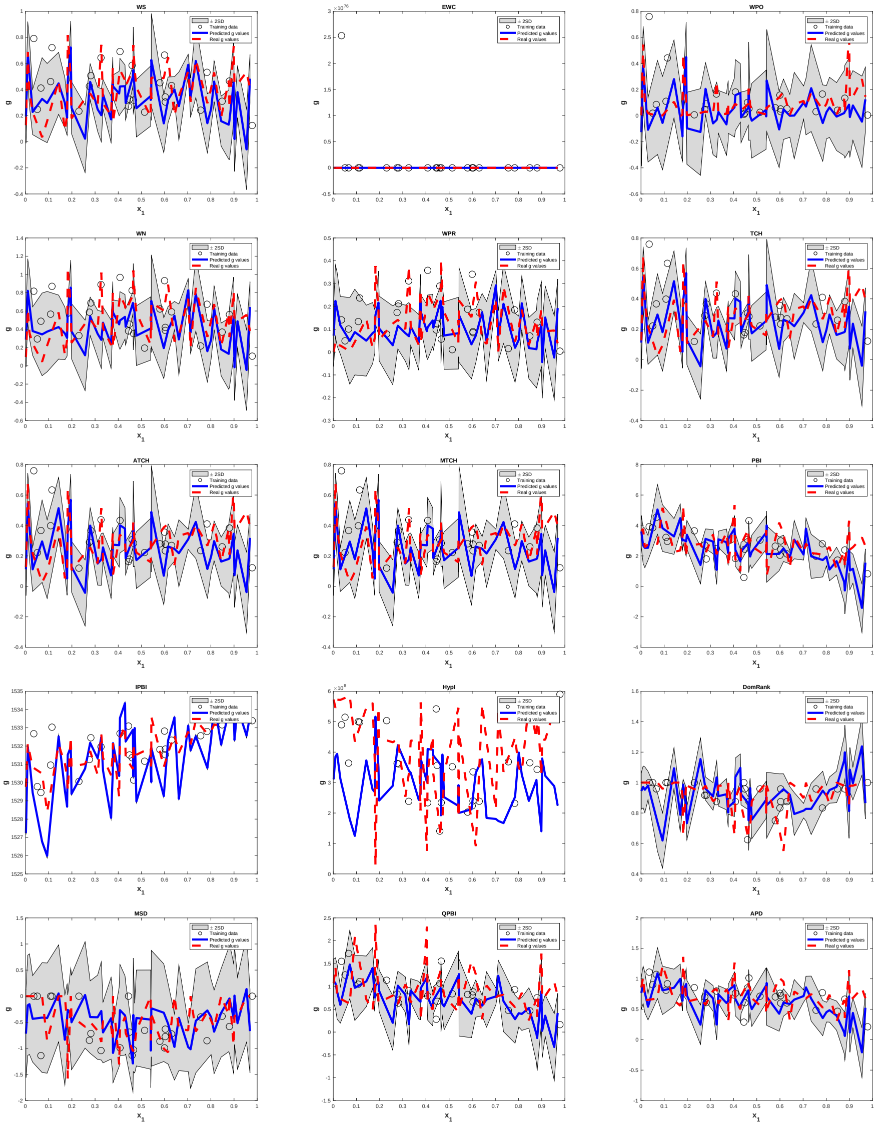


Figure 26: Scalarizing function values (notated by g) with one decision variable value for DTLZ3 three objectives, ±2SD represents the predicted g values with ± 2 standard deviations or uncertainty of the predicted values

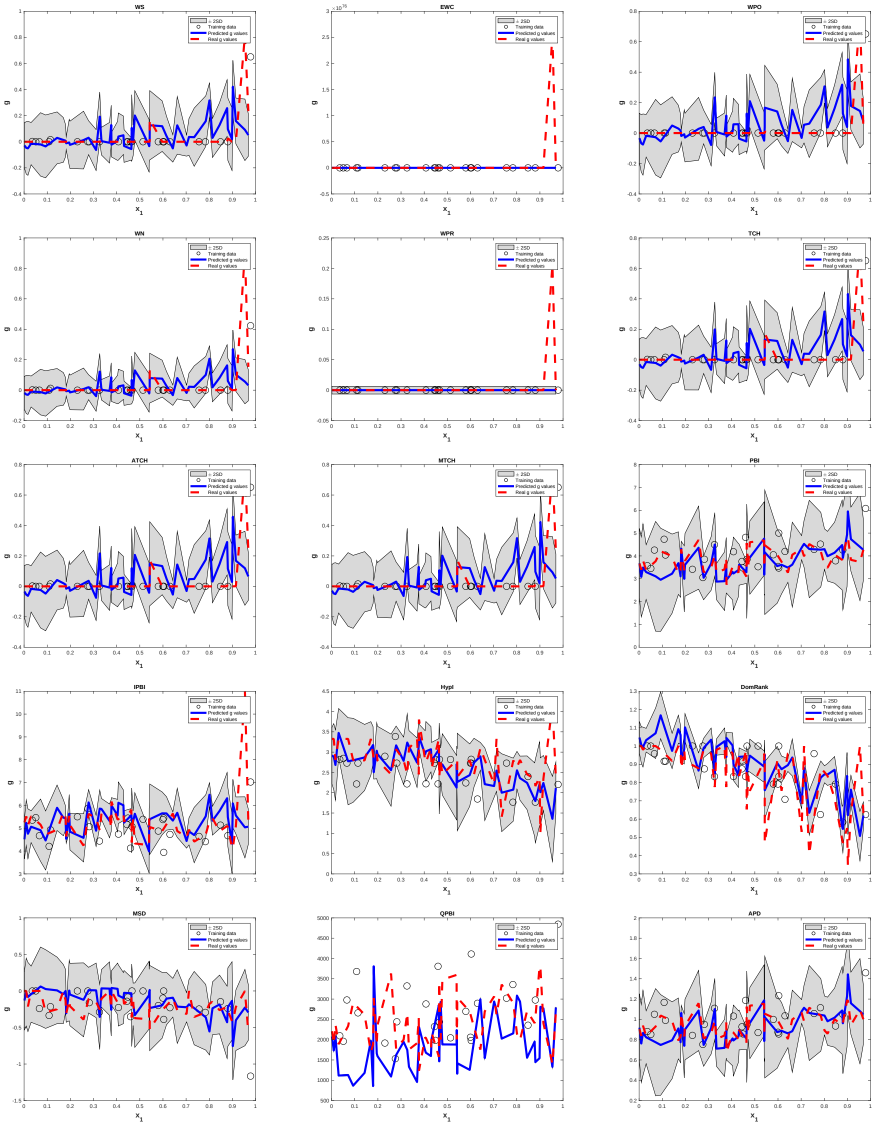


Figure 27: Scalarizing function values (notated by g) with one decision variable value for DTLZ4 three objectives, ±2SD represents the predicted g values with ± 2 standard deviations or uncertainty of the predicted values

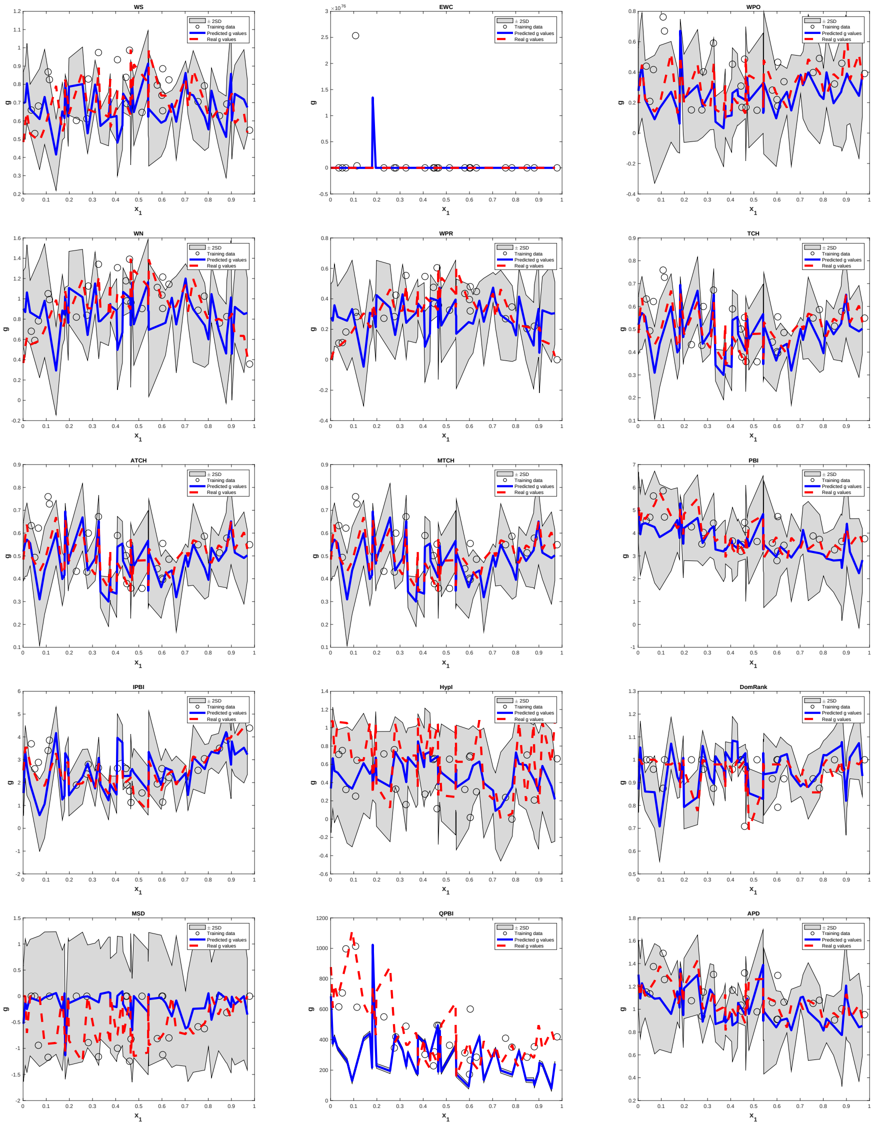


Figure 28: Scalarizing function values (notated by g) with one decision variable value for DTLZ5 three objectives, ±2SD represents the predicted g values with ± 2 standard deviations or uncertainty of the predicted values

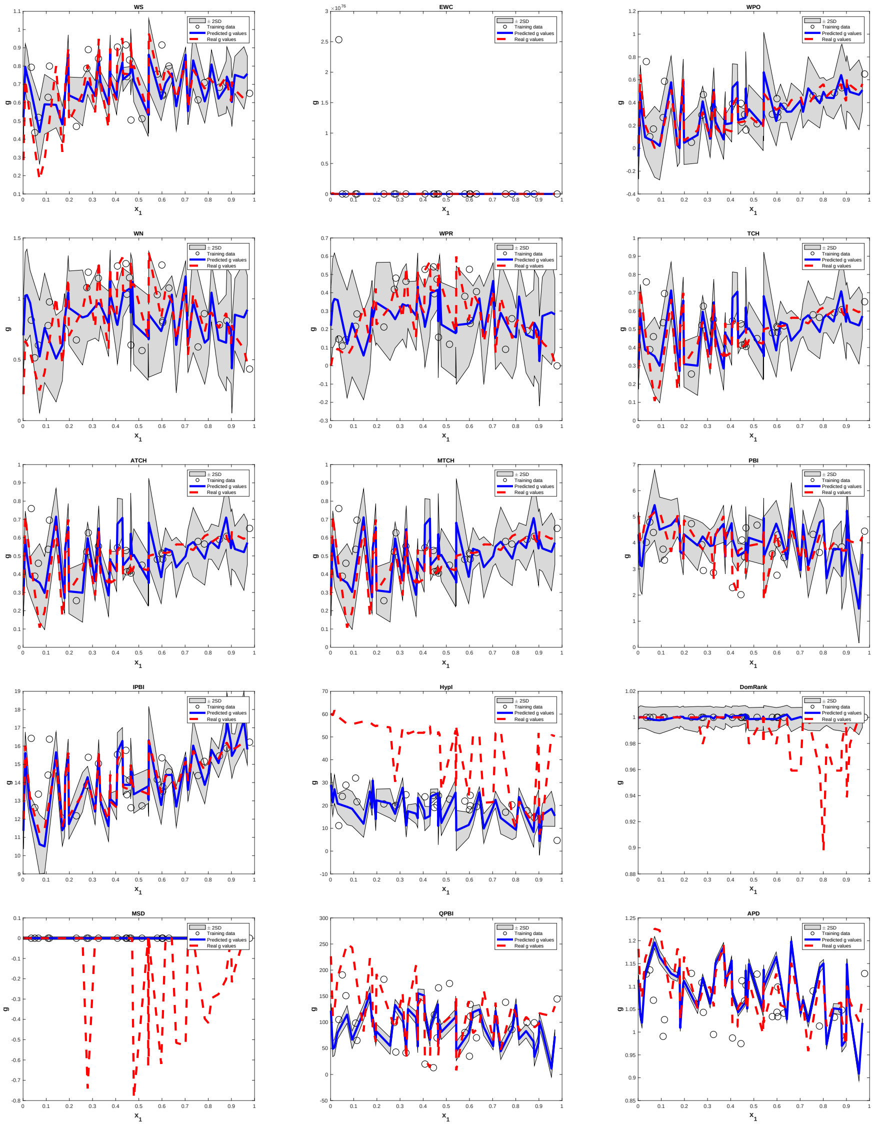


Figure 29: Scalarizing function values (notated by g) with one decision variable value for DTLZ6 three objectives, ±2SD represents the predicted g values with ± 2 standard deviations or uncertainty of the predicted values

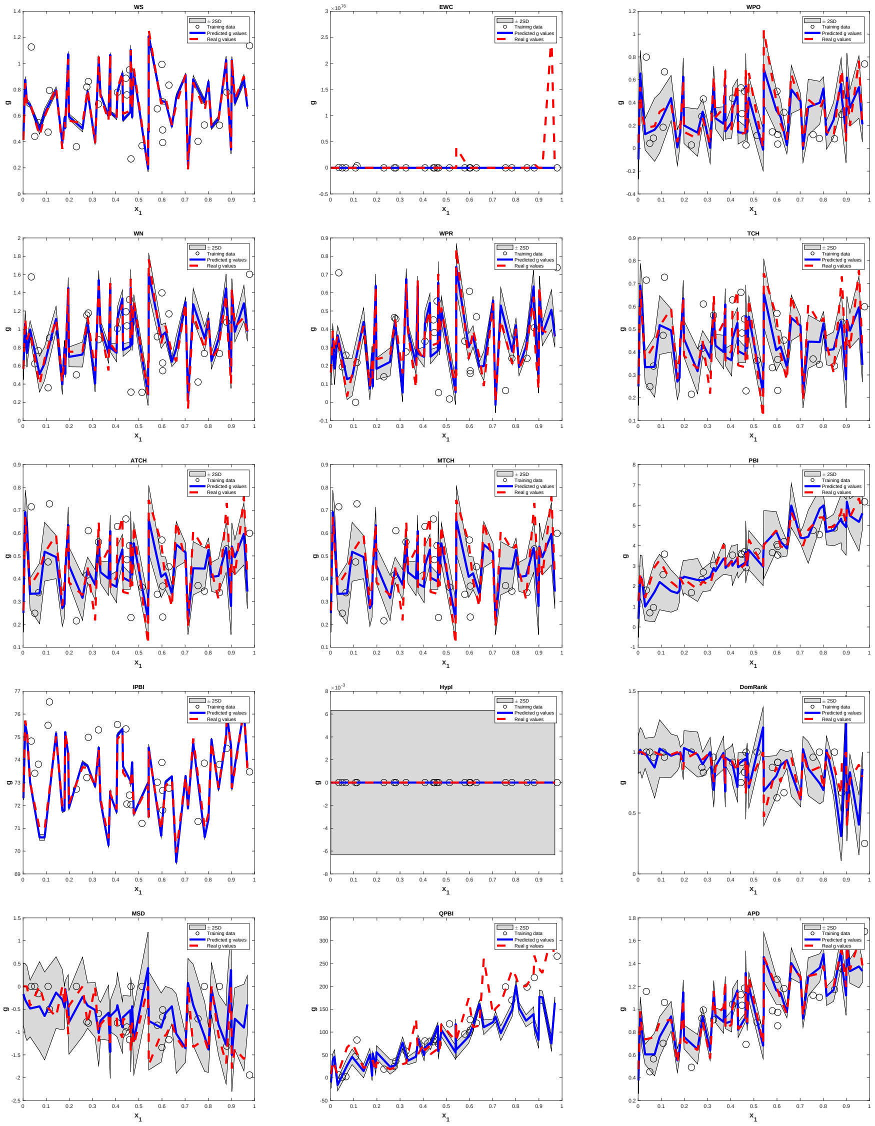

Figure 30: Scalarizing function values (notated by g) with one decision variable value for DTLZ7 three objectives, ±2SD represents the predicted g values with ± 2 standard deviations or uncertainty of the predicted values

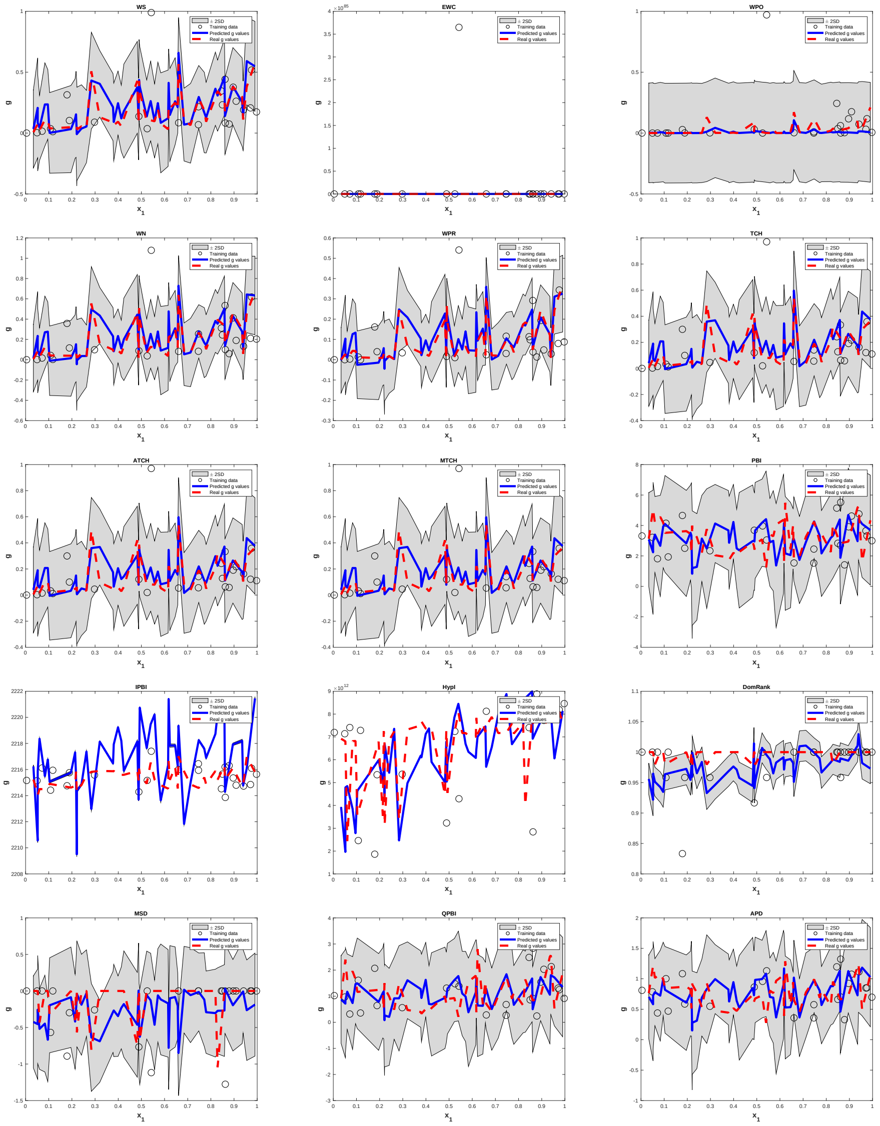


Figure 31: Scalarizing function values (notated by g) with one decision variable value for DTLZ1 five objectives, ±2SD represents the predicted g values with ± 2 standard deviations or uncertainty of the predicted values

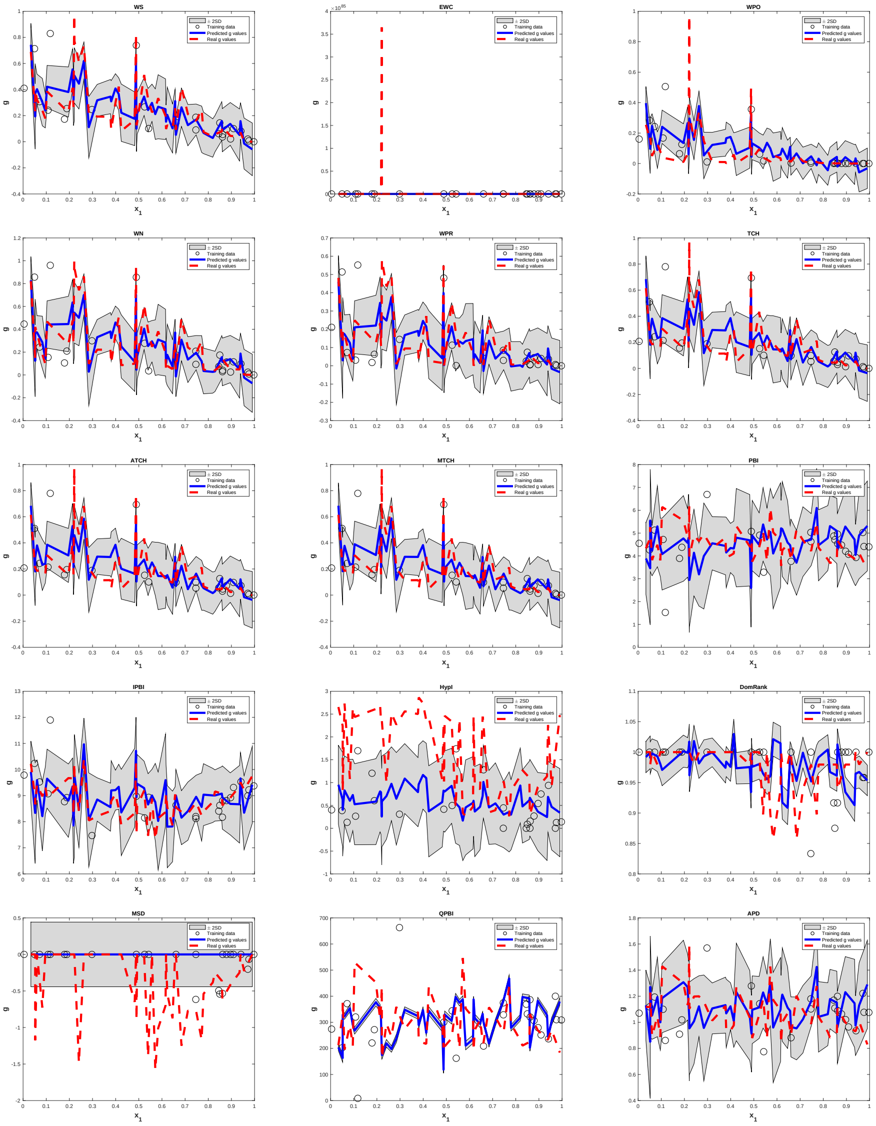


Figure 32: Scalarizing function values (notated by g) with one decision variable value for DTLZ2 five objectives, ±2SD represents the predicted g values with ± 2 standard deviations or uncertainty of the predicted values

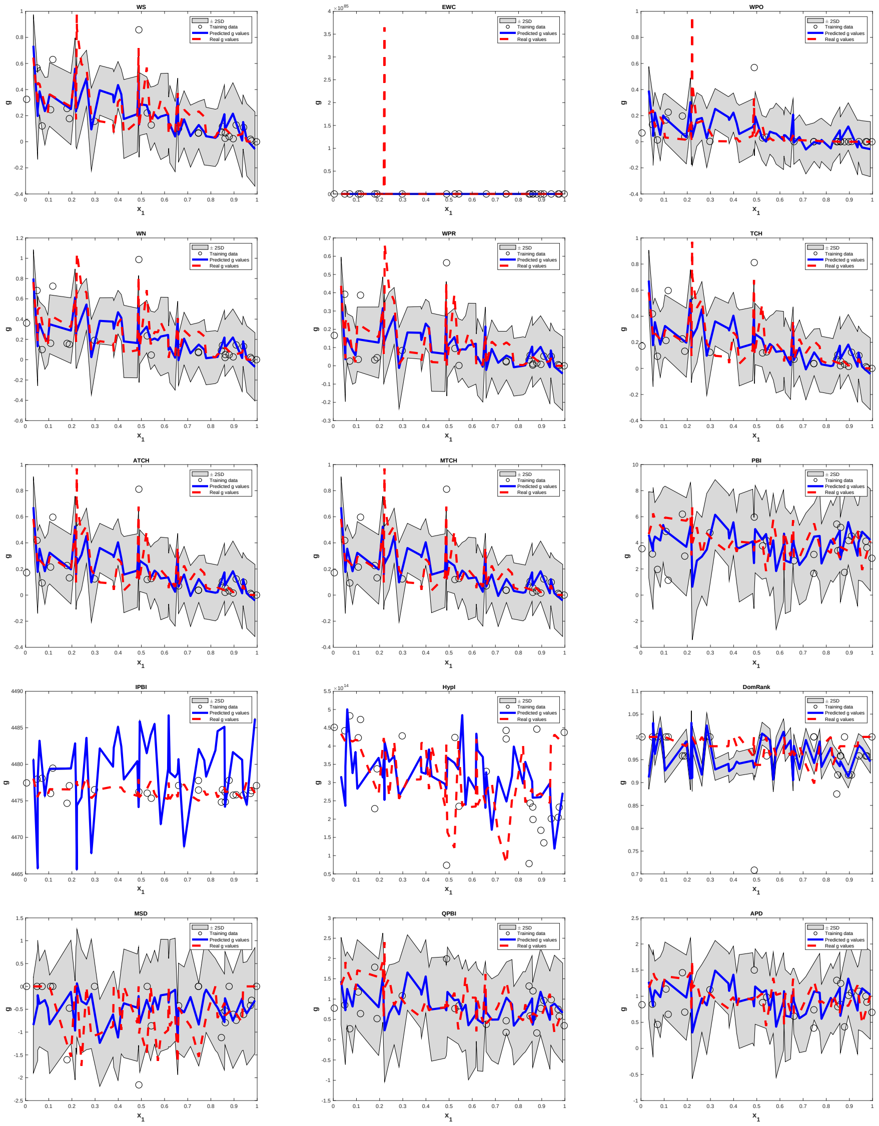


Figure 33: Scalarizing function values (notated by g) with one decision variable value for DTLZ3 five objectives, ±2SD represents the predicted g values with ± 2 standard deviations or uncertainty of the predicted values

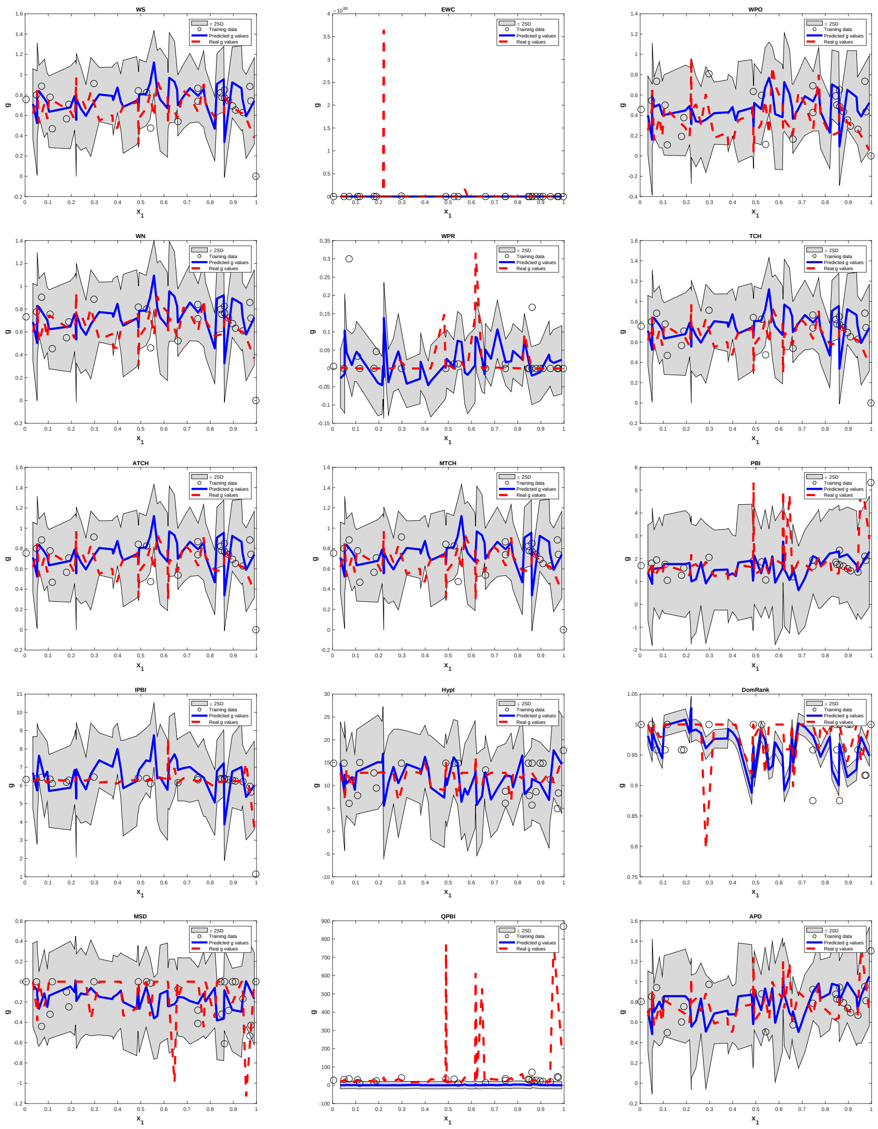


Figure 34: Scalarizing function values (notated by g) with one decision variable value for DTLZ4 five objectives, ±2SD represents the predicted g values with ± 2 standard deviations or uncertainty of the predicted values

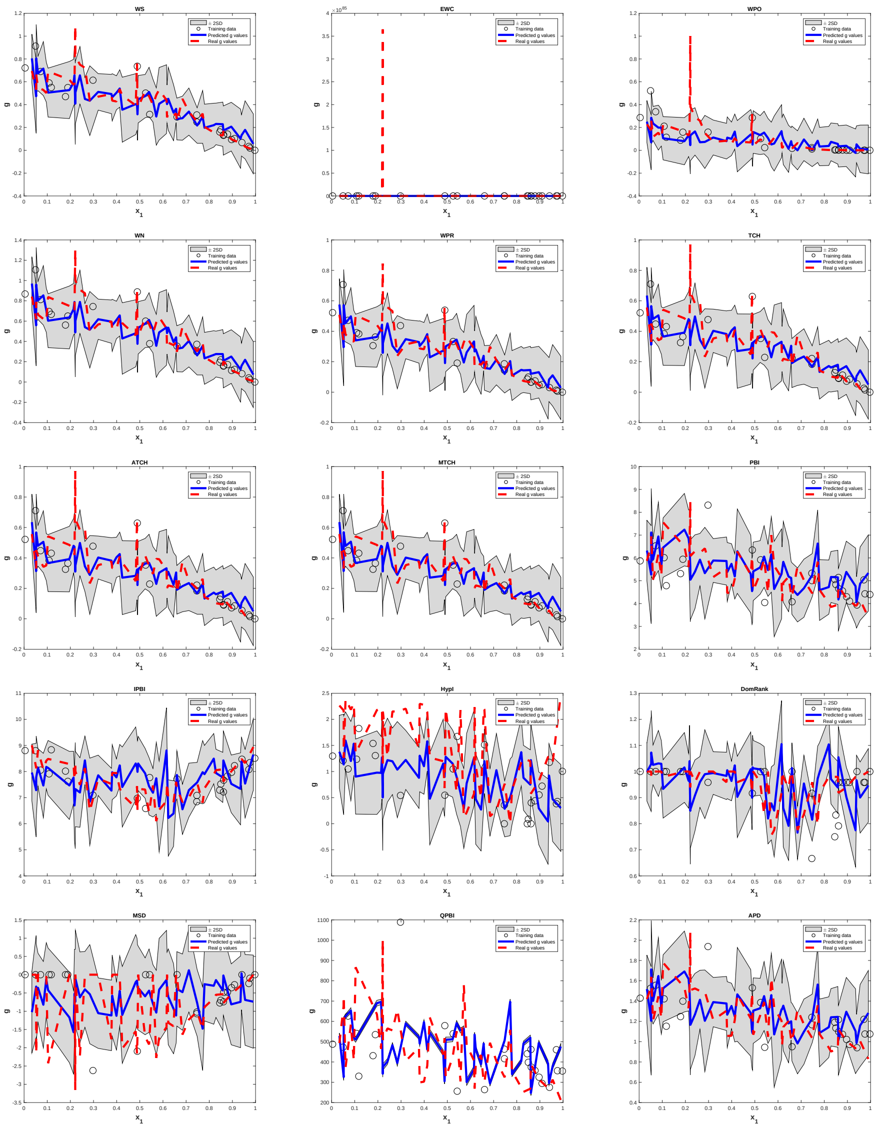


Figure 35: Scalarizing function values (notated by g) with one decision variable value for DTLZ5 five objectives, ±2SD represents the predicted g values with ± 2 standard deviations or uncertainty of the predicted values

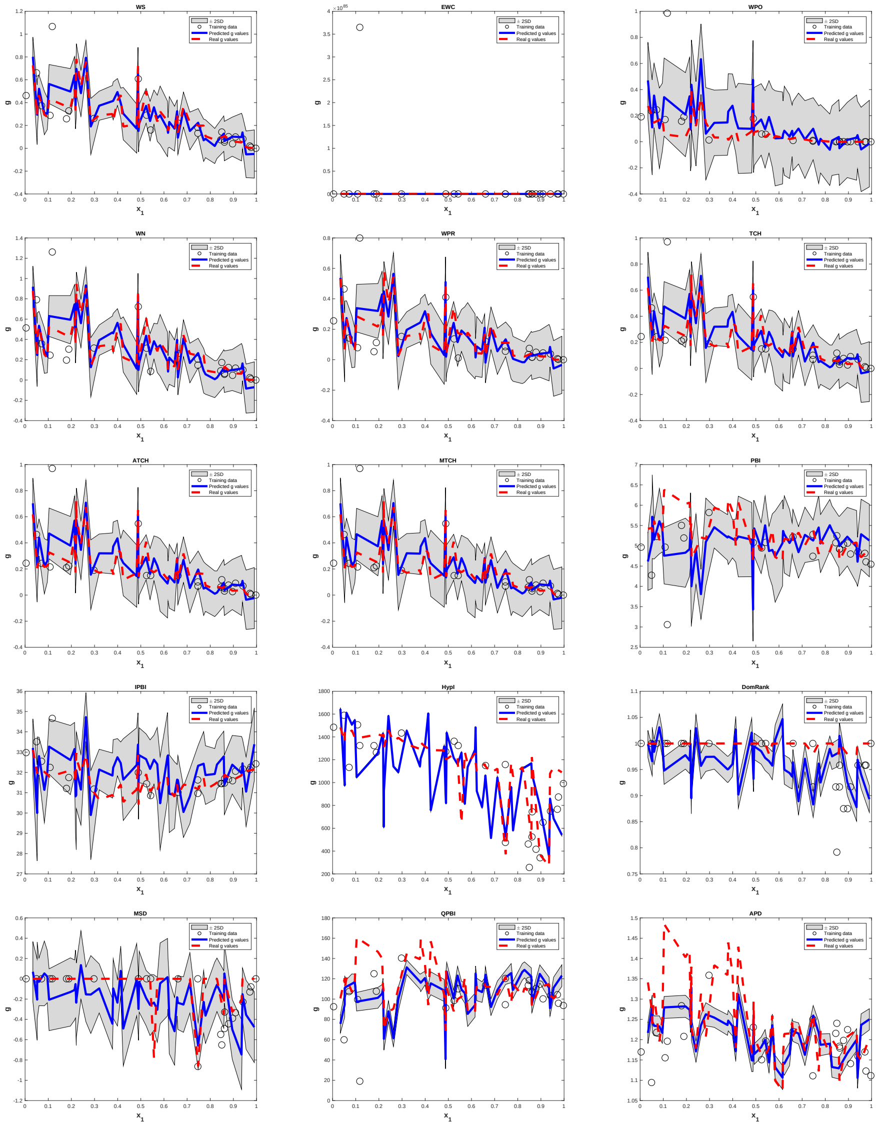


Figure 36: Scalarizing function values (notated by g) with one decision variable value for DTLZ6 five objectives, ±2SD represents the predicted g values with ± 2 standard deviations or uncertainty of the predicted values

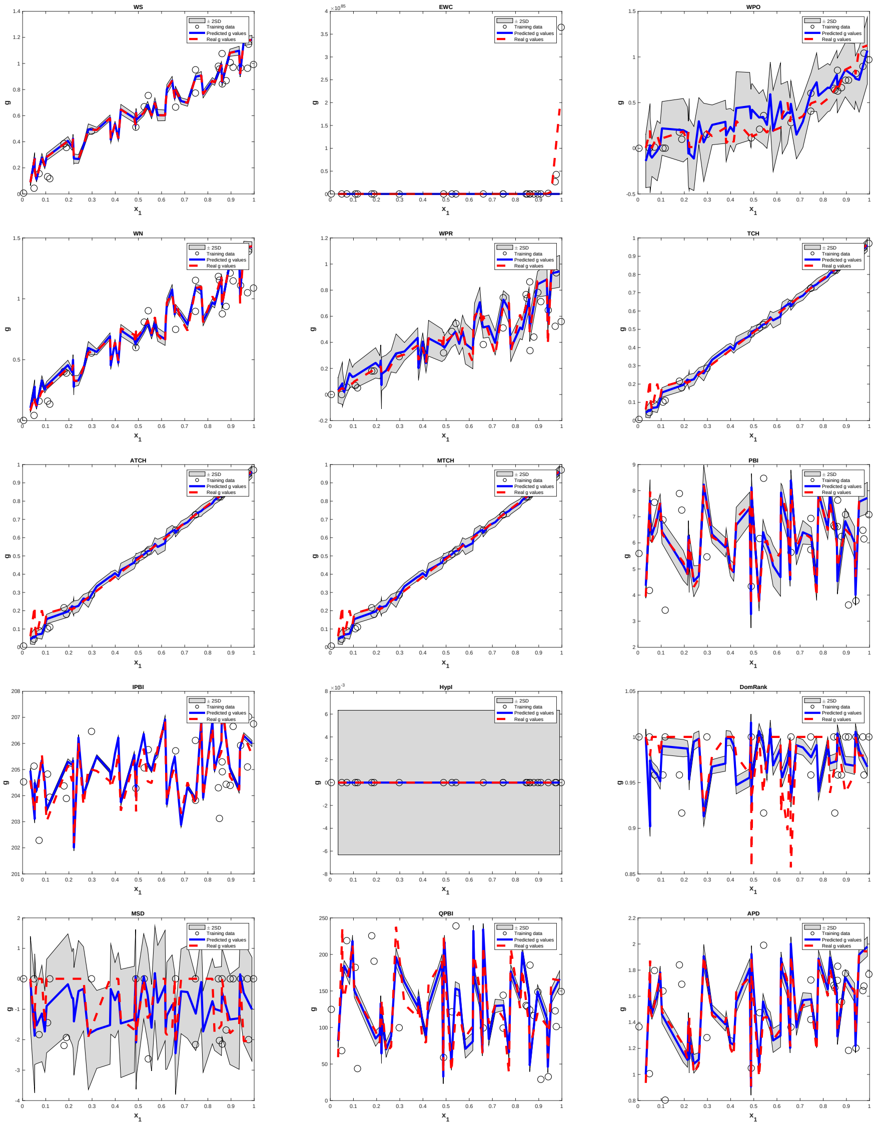


Figure 37: Scalarizing function values (notated by g) with one decision variable value for DTLZ7 five objectives, ±2SD represents the predicted g values with ± 2 standard deviations or uncertainty of the predicted values

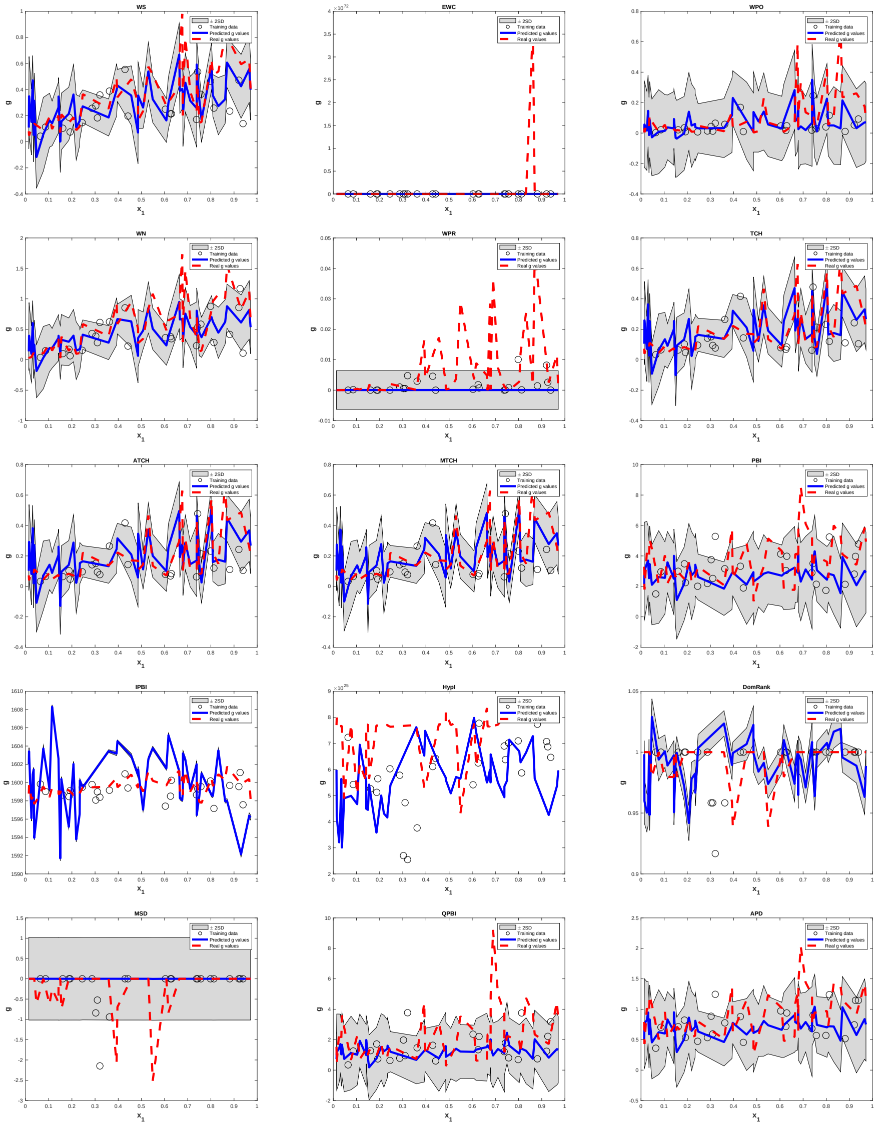

Figure 38: Scalarizing function values (notated by g) with one decision variable value for DTLZ1 10 objectives, ±2SD represents the predicted g values with ± 2 standard deviations or uncertainty of the predicted values

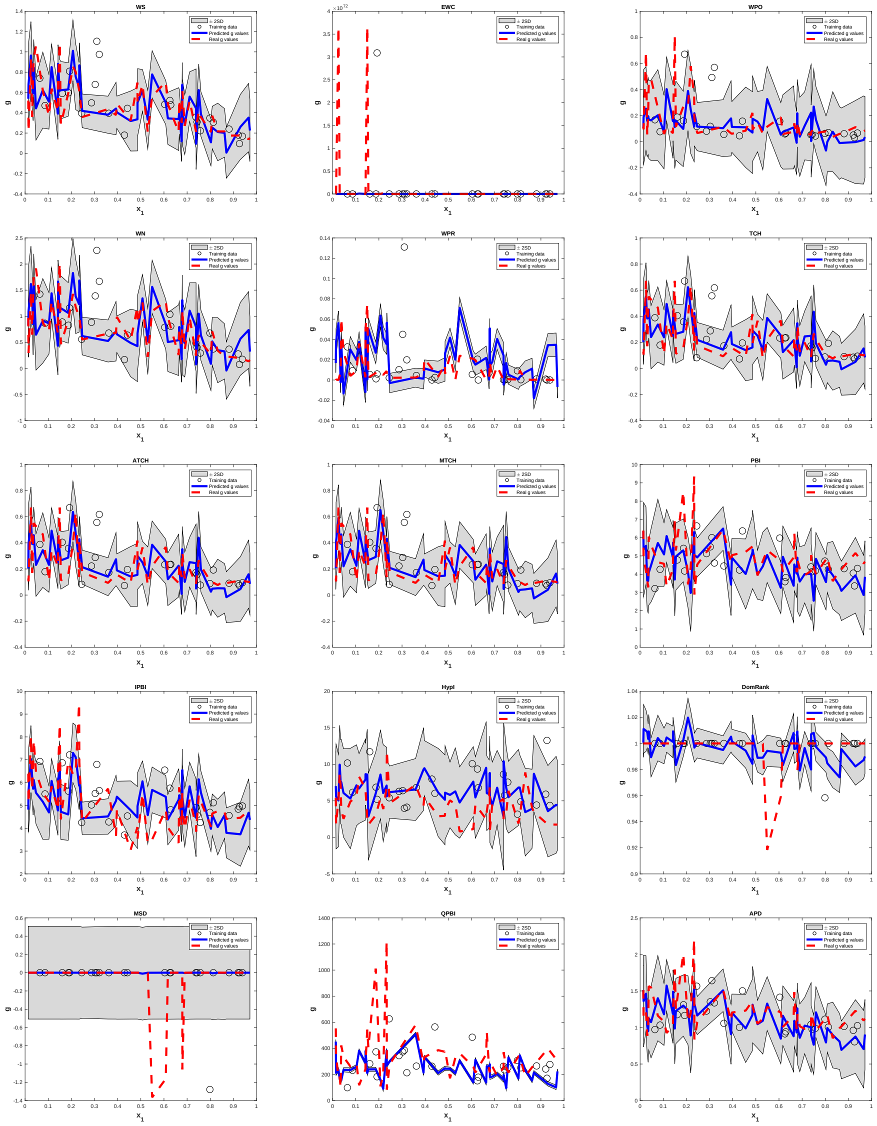

Figure 39: Scalarizing function values (notated by g) with one decision variable value for DTLZ2 10 objectives, ±2SD represents the predicted g values with ± 2 standard deviations or uncertainty of the predicted values

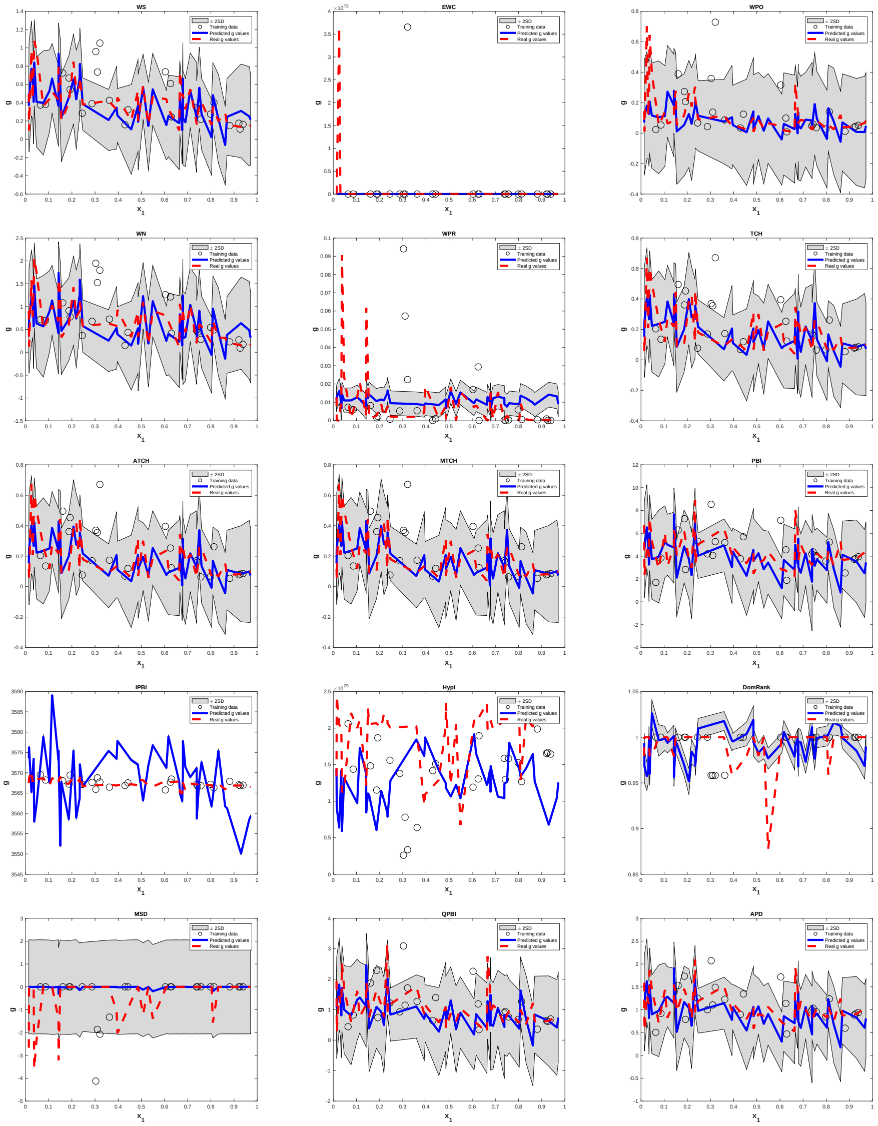


Figure 40: Scalarizing function values (notated by g) with one decision variable value for DTLZ3 10 objectives, ±2SD represents the predicted g values with ± 2 standard deviations or uncertainty of the predicted values

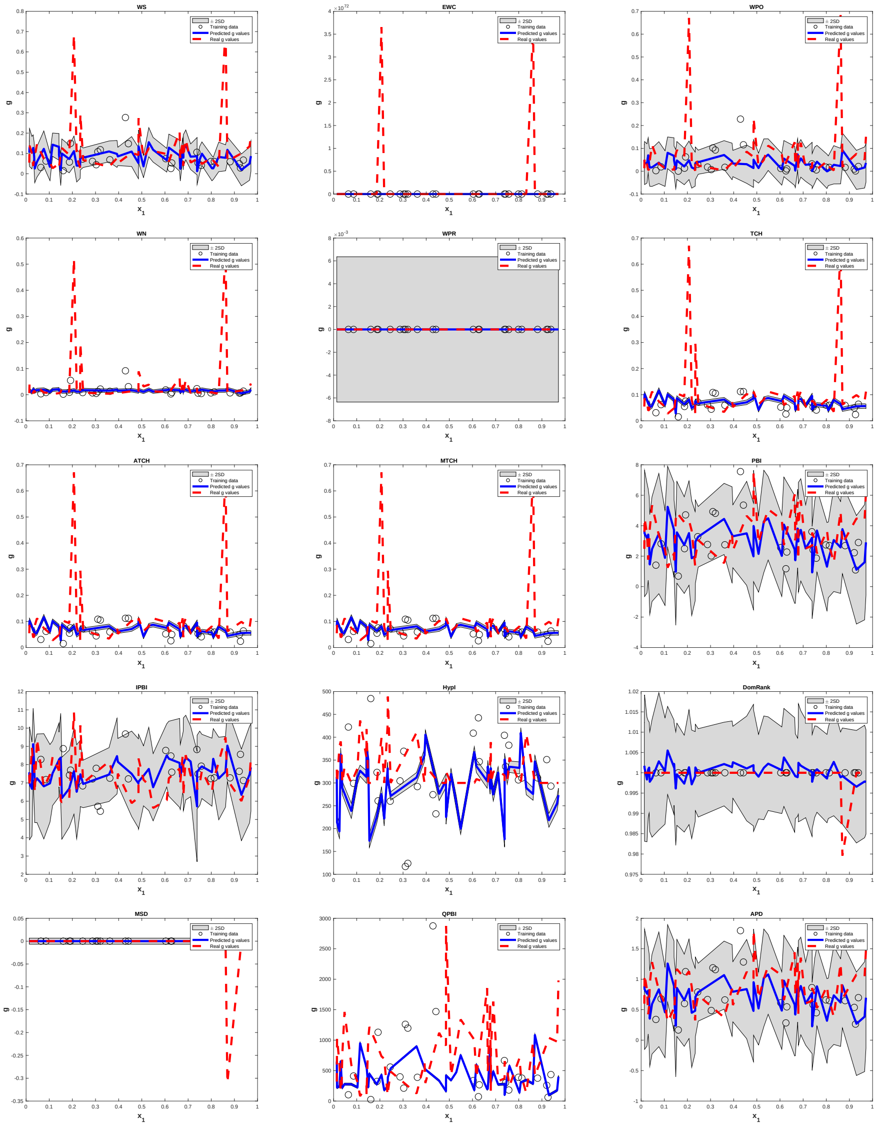


Figure 41: Scalarizing function values (notated by g) with one decision variable value for DTLZ4 10 objectives, ±2SD represents the predicted g values with ± 2 standard deviations or uncertainty of the predicted values

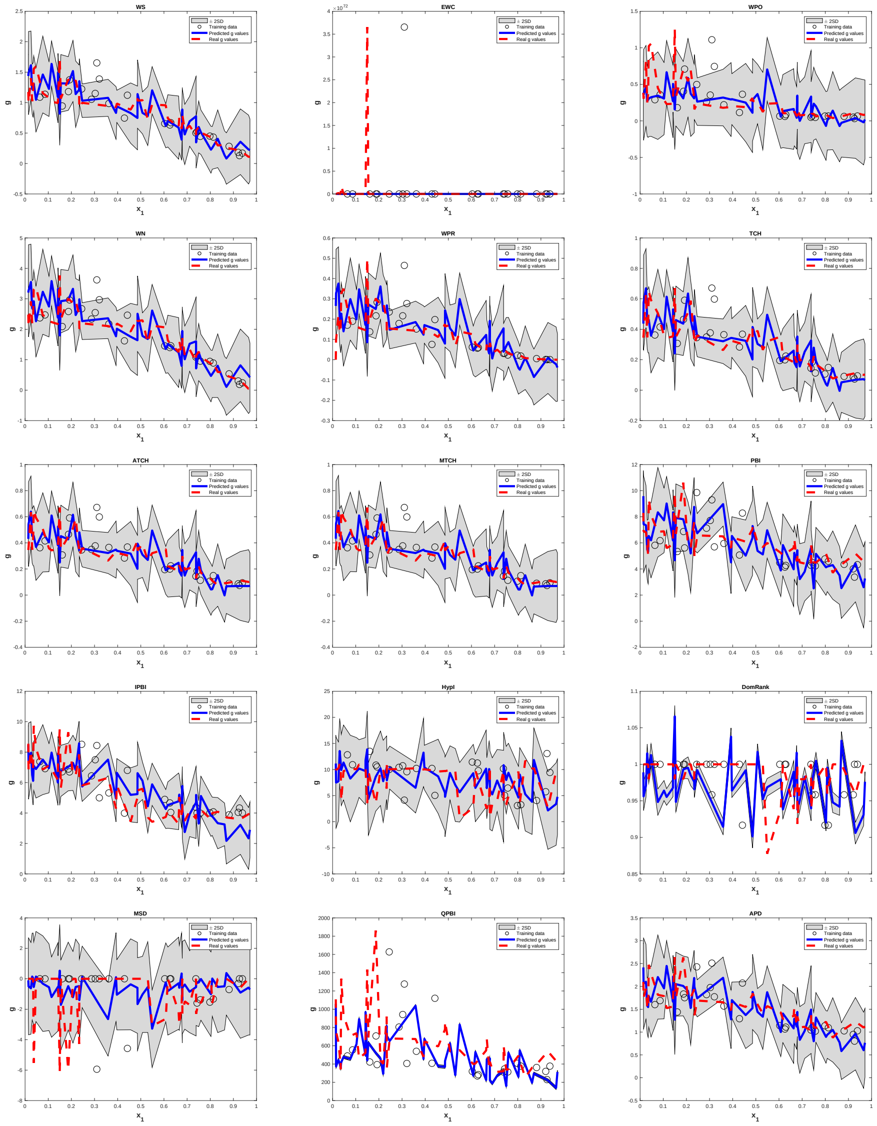


Figure 42: Scalarizing function values (notated by g) with one decision variable value for DTLZ5 10 objectives, ±2SD represents the predicted g values with ± 2 standard deviations or uncertainty of the predicted values

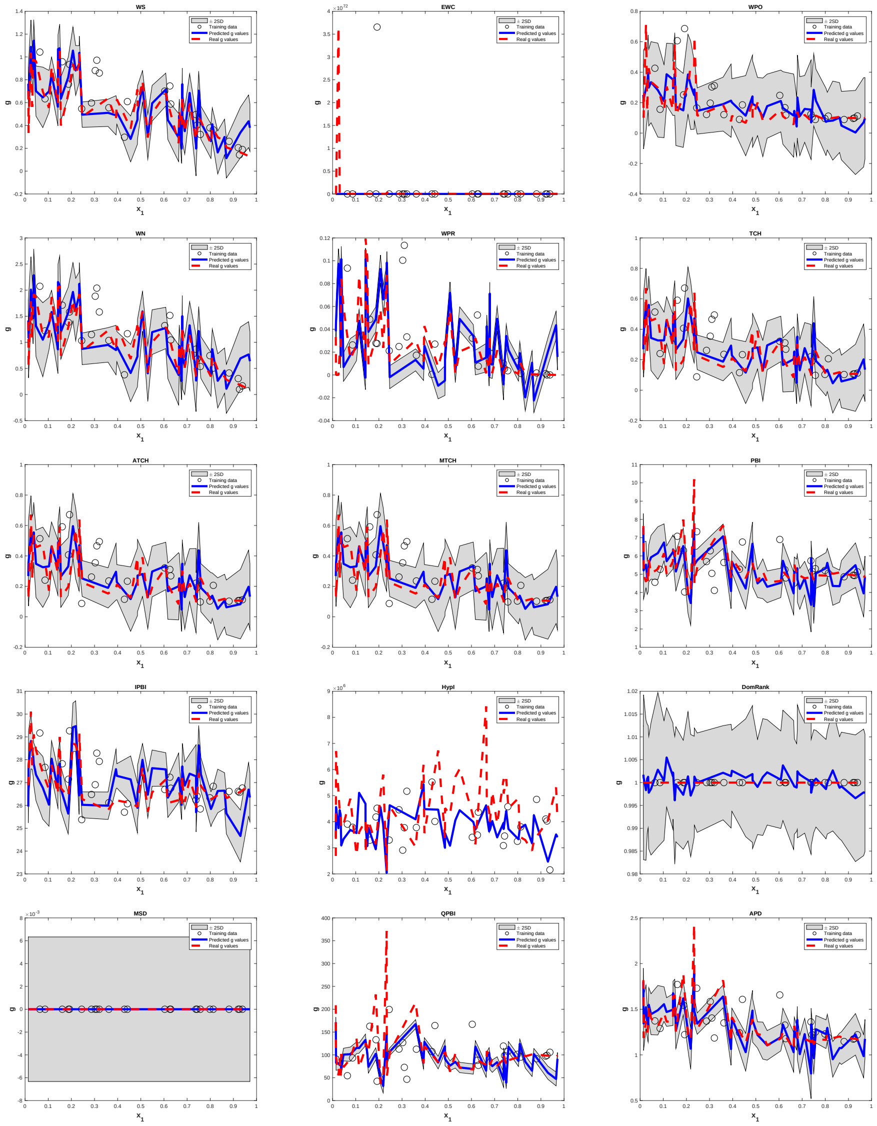


Figure 43: Scalarizing function values (notated by g) with one decision variable value for DTLZ6 10 objectives, ±2SD represents the predicted g values with ± 2 standard deviations or uncertainty of the predicted values

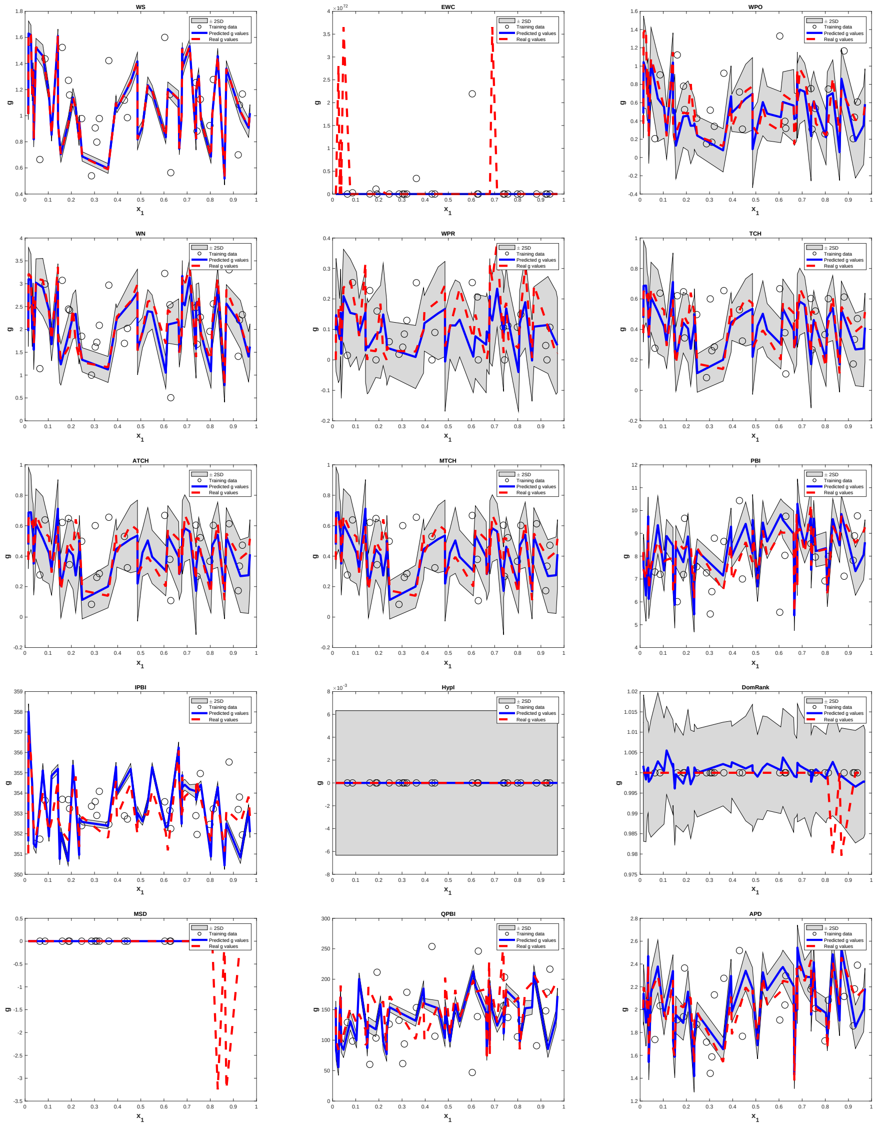

Figure 44: Scalarizing function values (notated by g) with one decision variable value for DTLZ7 10 objectives, ±2SD represents the predicted g values with ± 2 standard deviations or uncertainty of the predicted values
