# Supplementary material for: Scalarizing Functions in Bayesian Multiobjective Optimization
Source: arXiv:1904.05760 source file (2019-04-11)
Supplement: Supplementary file 2 [file Supplementary_material.tex]

Supplementary material

\section{Supplementary material}

\subsection{Sensitivity of HypI towards reference point}

\subsection{Sensitivity of function towards the number of objectives}

\subsection{Approximated Pareto fronts}
